# Supplementary material for: Achieving Pareto Optimality using Efficient Parameter Reduction for DNNs in Resource-Constrained Edge Environment
Source: arXiv:2403.10569 source file (2024-03-14)
Supplement: Supplementary file 1 [file appendix.tex]

\section{Appendix}

\setcounter{figure}{0} 

%Defect detection with pre-training
\begin{figure}[h!]
    \centering
  \subfloat[MobileNetV2: Open Circuit\label{3a}]{%
       \includegraphics[width=0.49\linewidth]{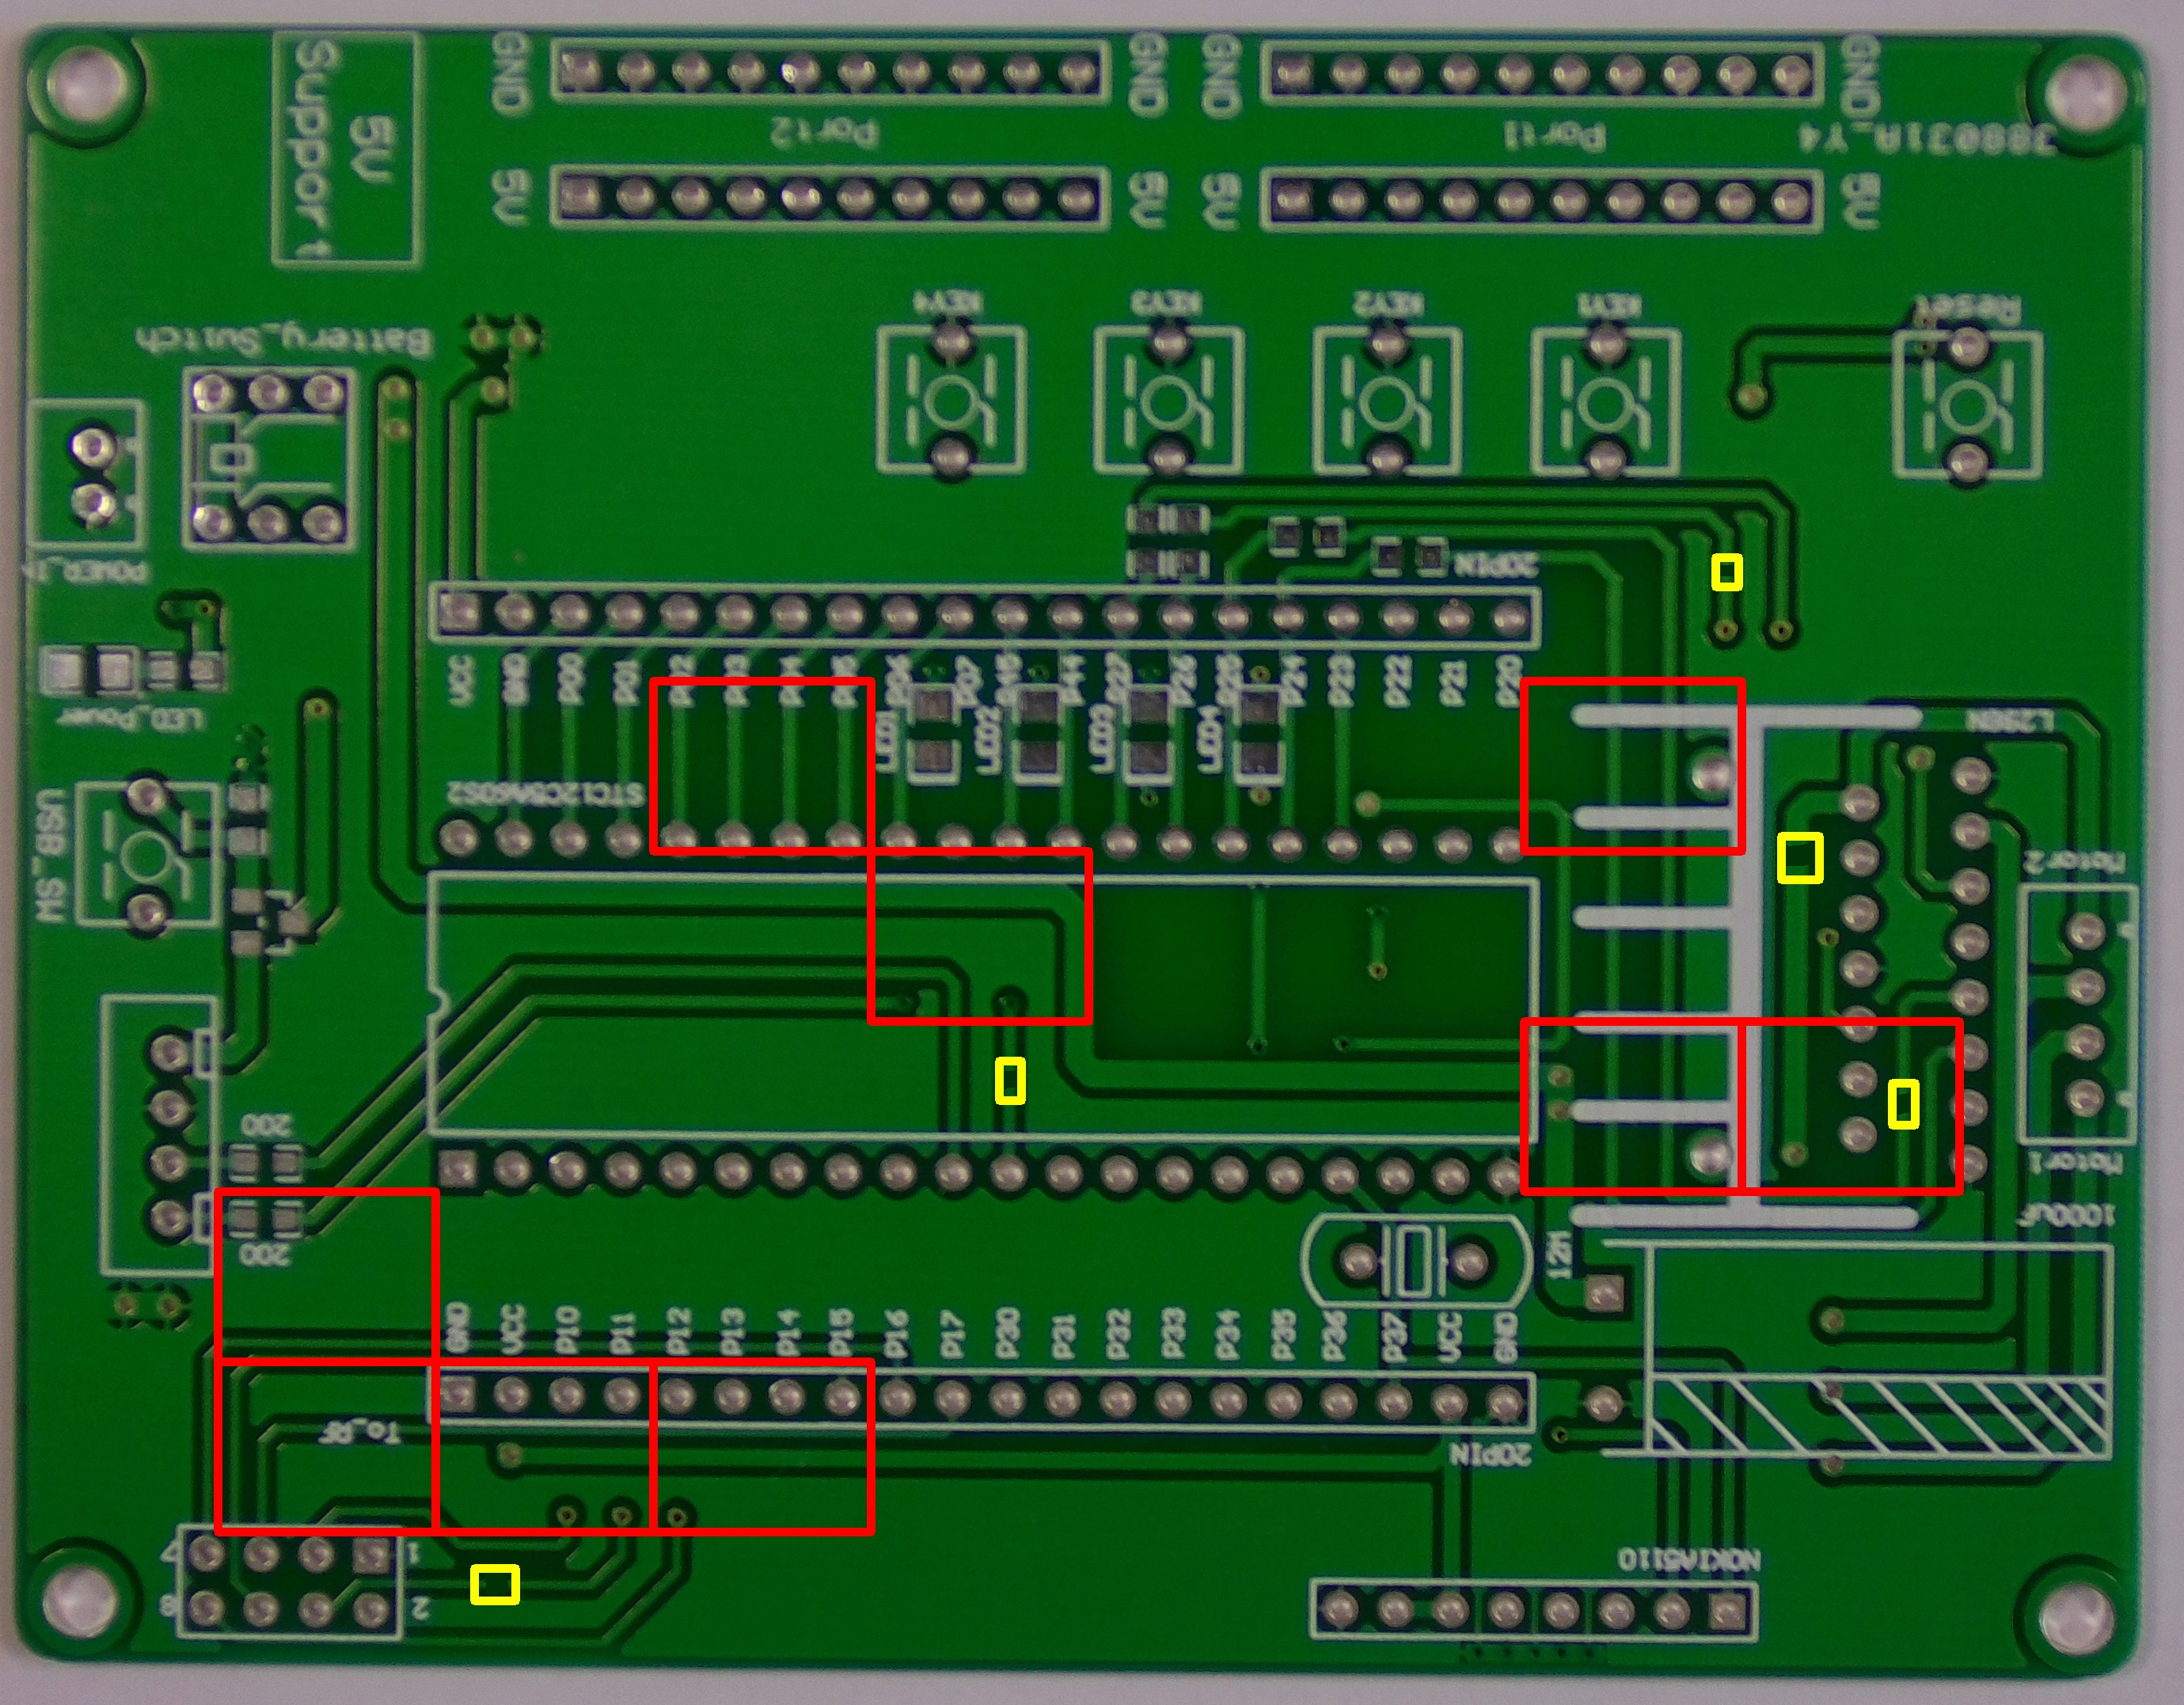}}
    \hfill
  \subfloat[MobileNetV2: Spur\label{3a}]{%
       \includegraphics[width=0.48\linewidth]{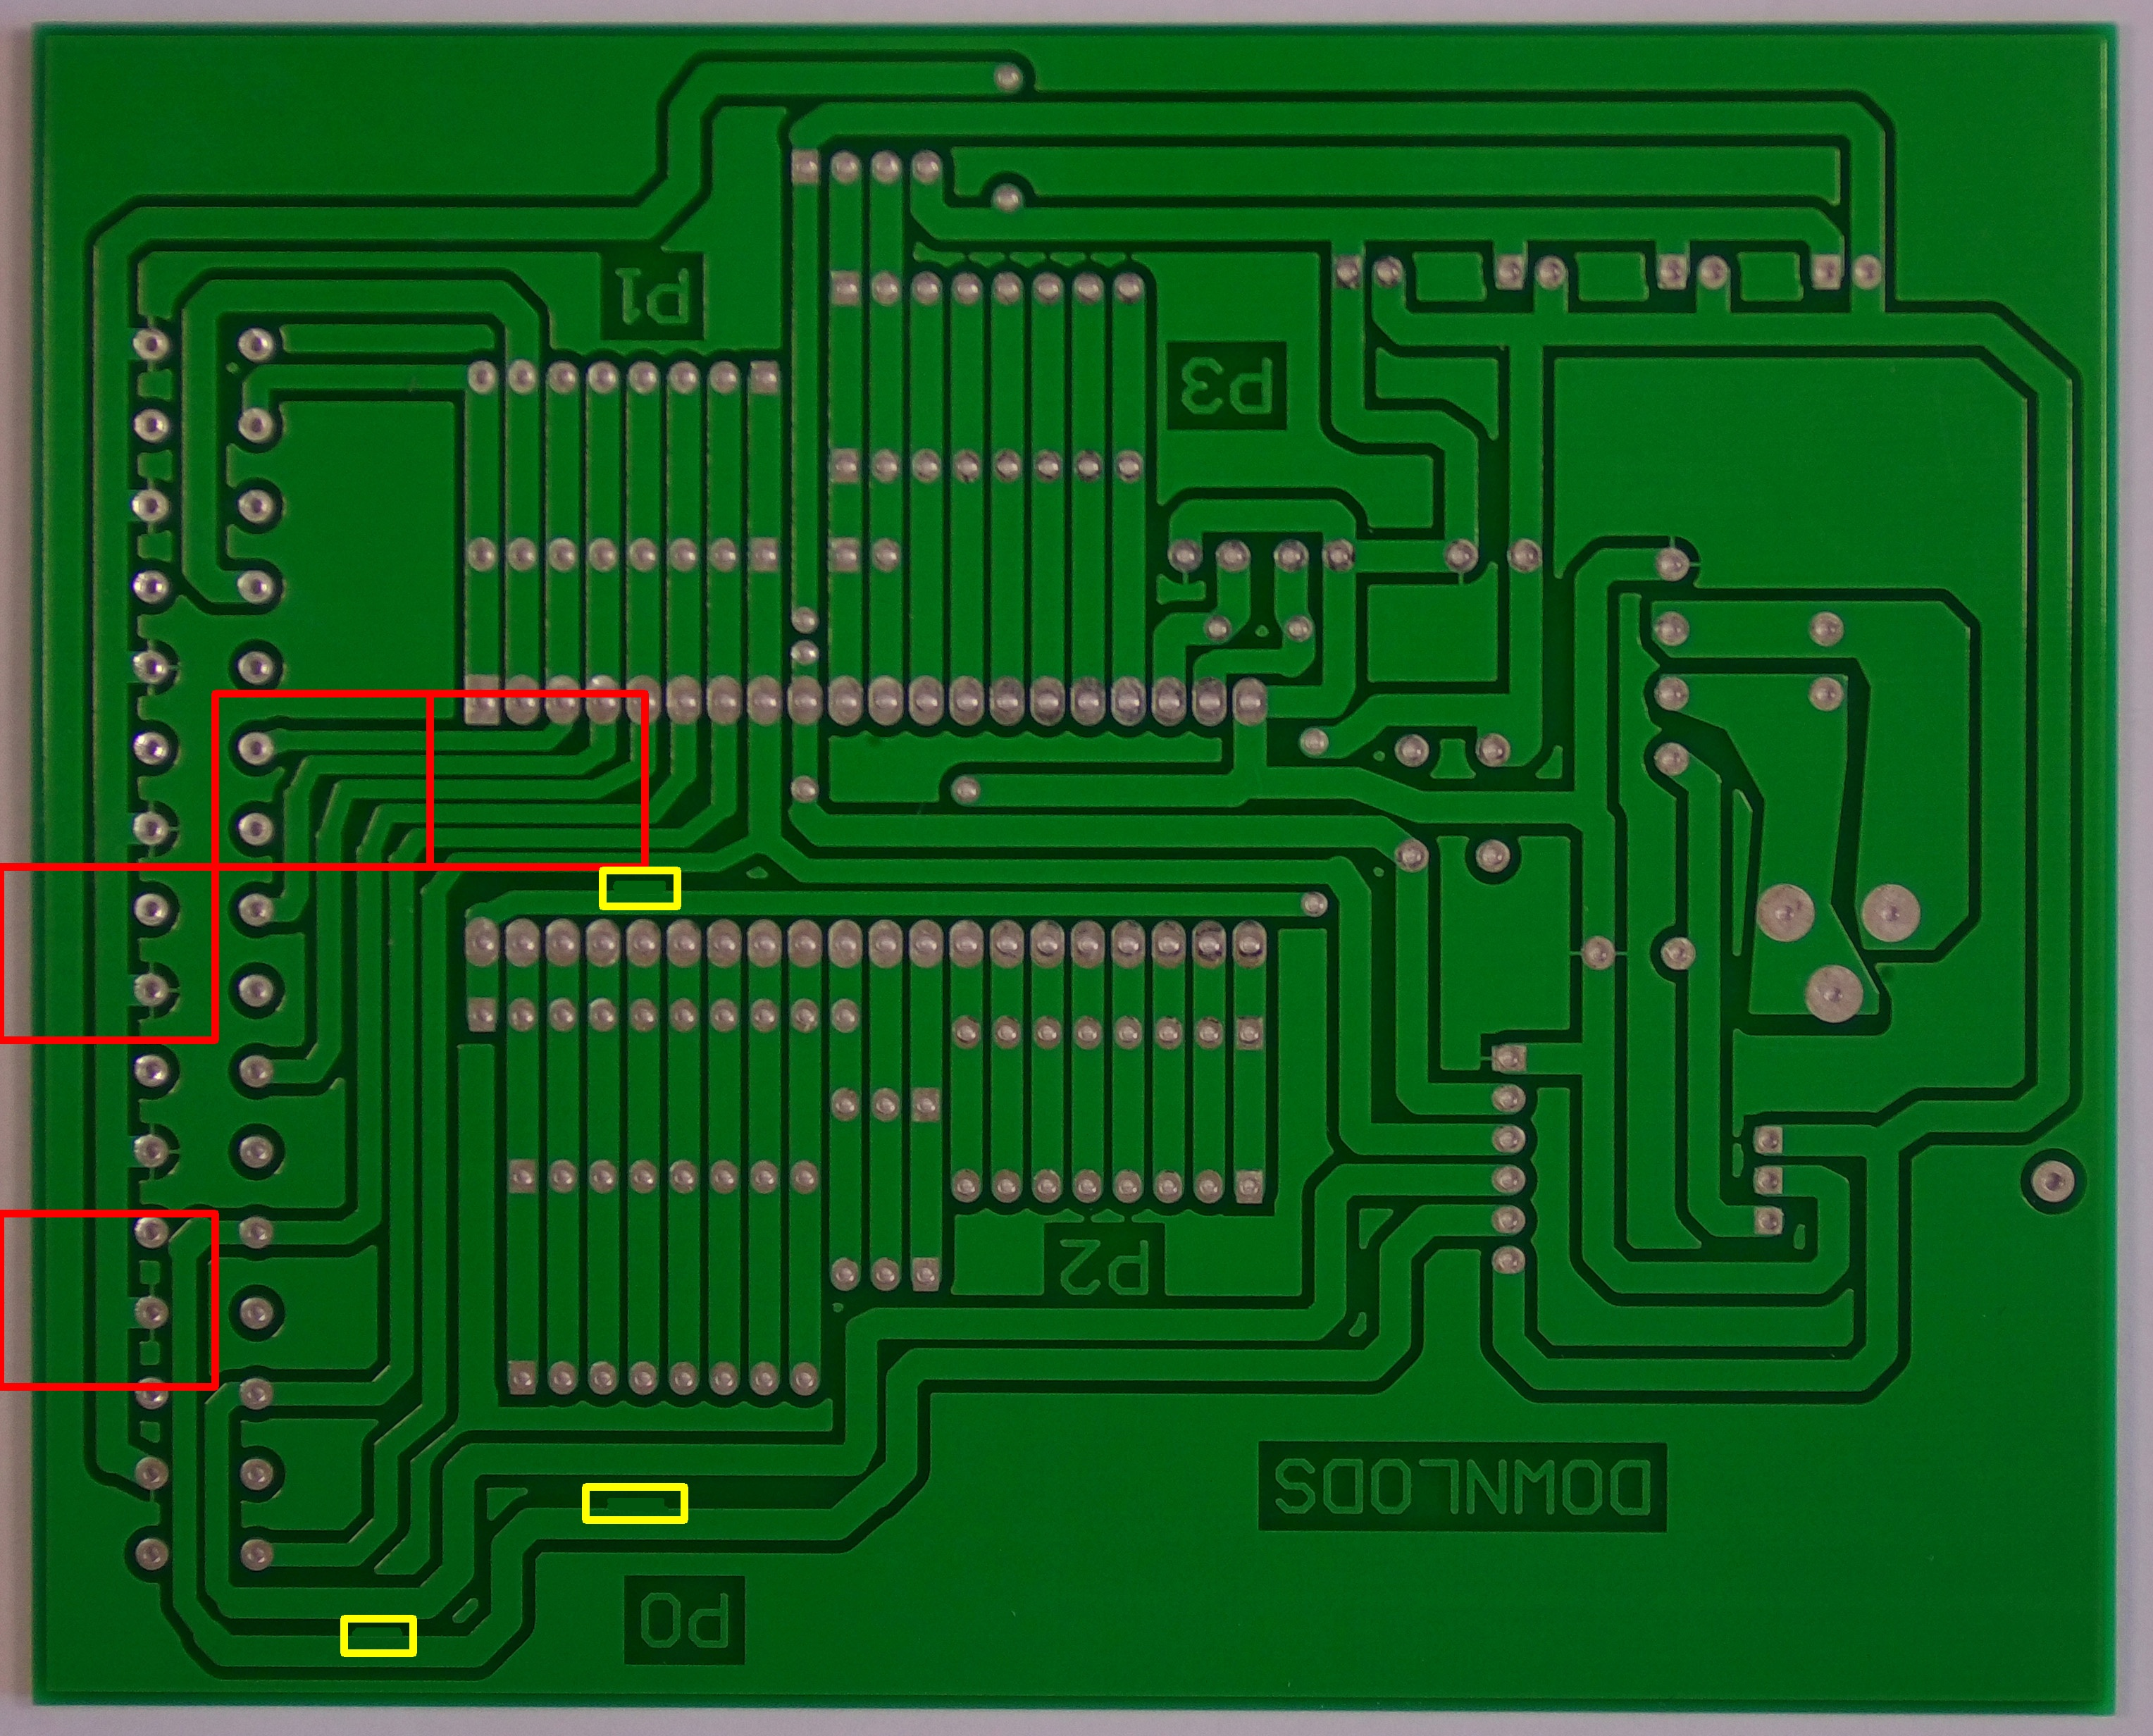}}
    \hfill
    
  \subfloat[EfficientNetV2B0: Open Circuit\label{6c}]{%
        \includegraphics[width=0.49\linewidth]{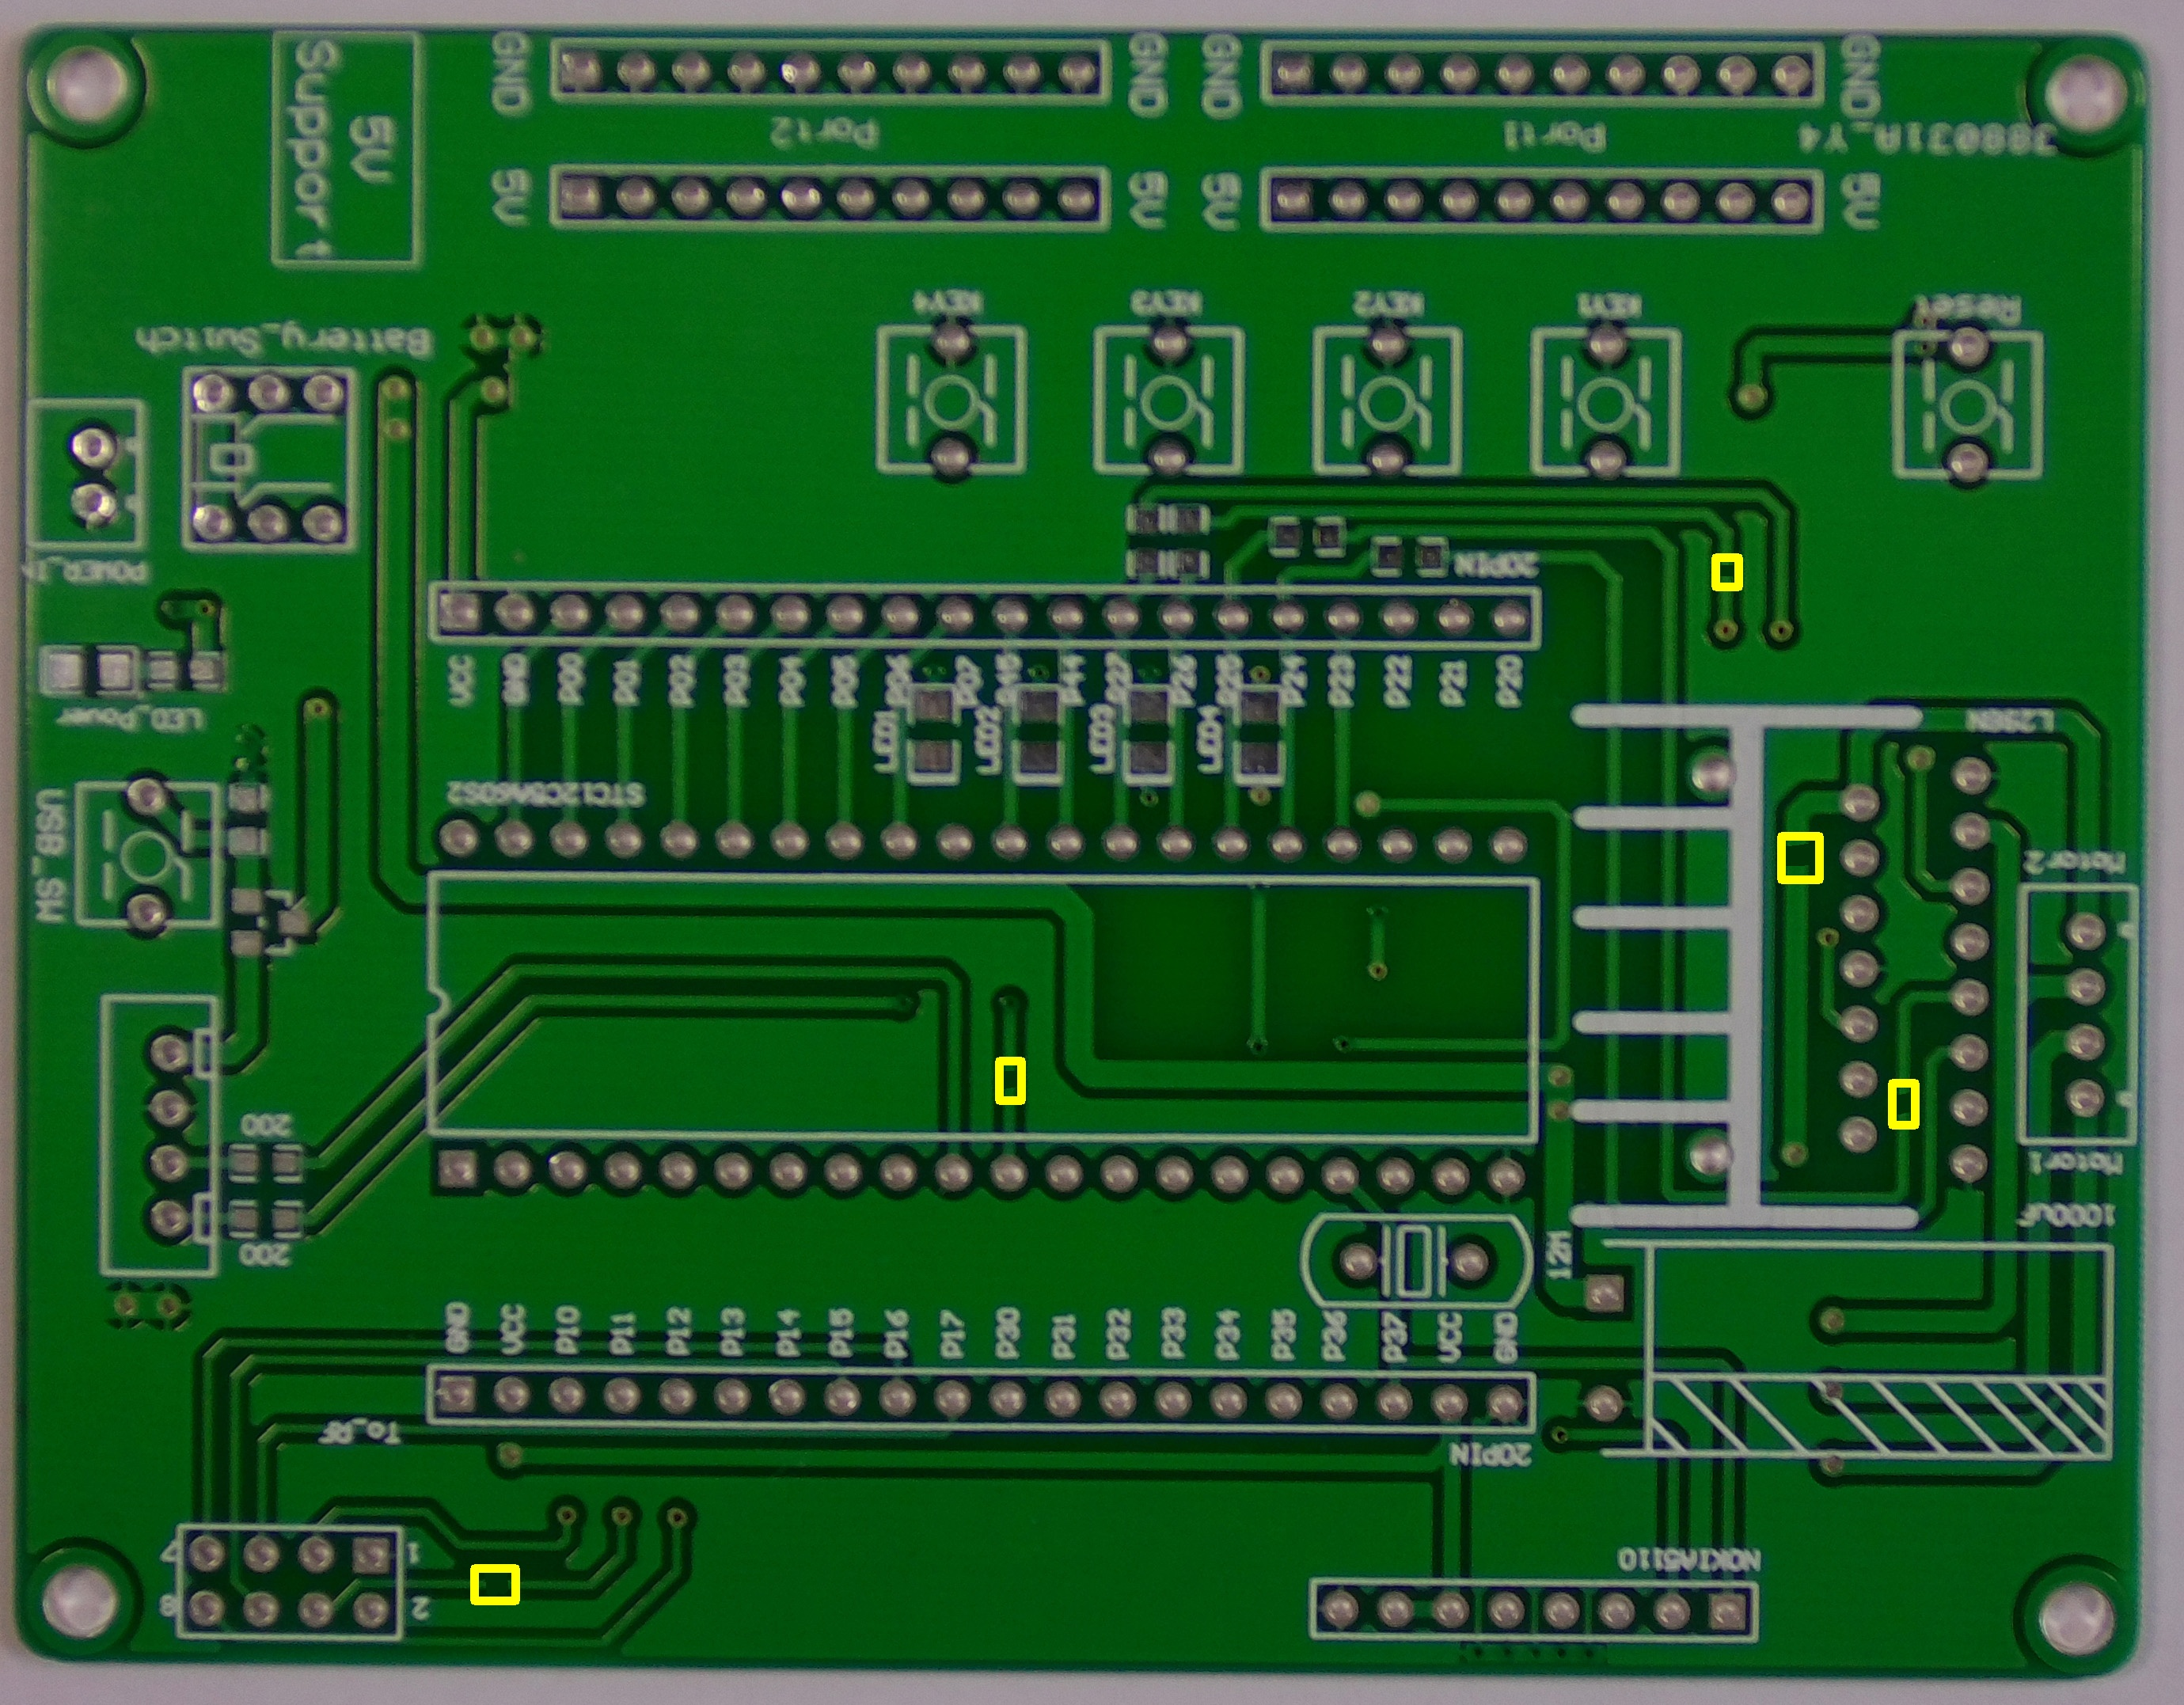}}
    \hfill
  \subfloat[EfficientNetV2B0: Spur\label{6c}]{%
        \includegraphics[width=0.48\linewidth]{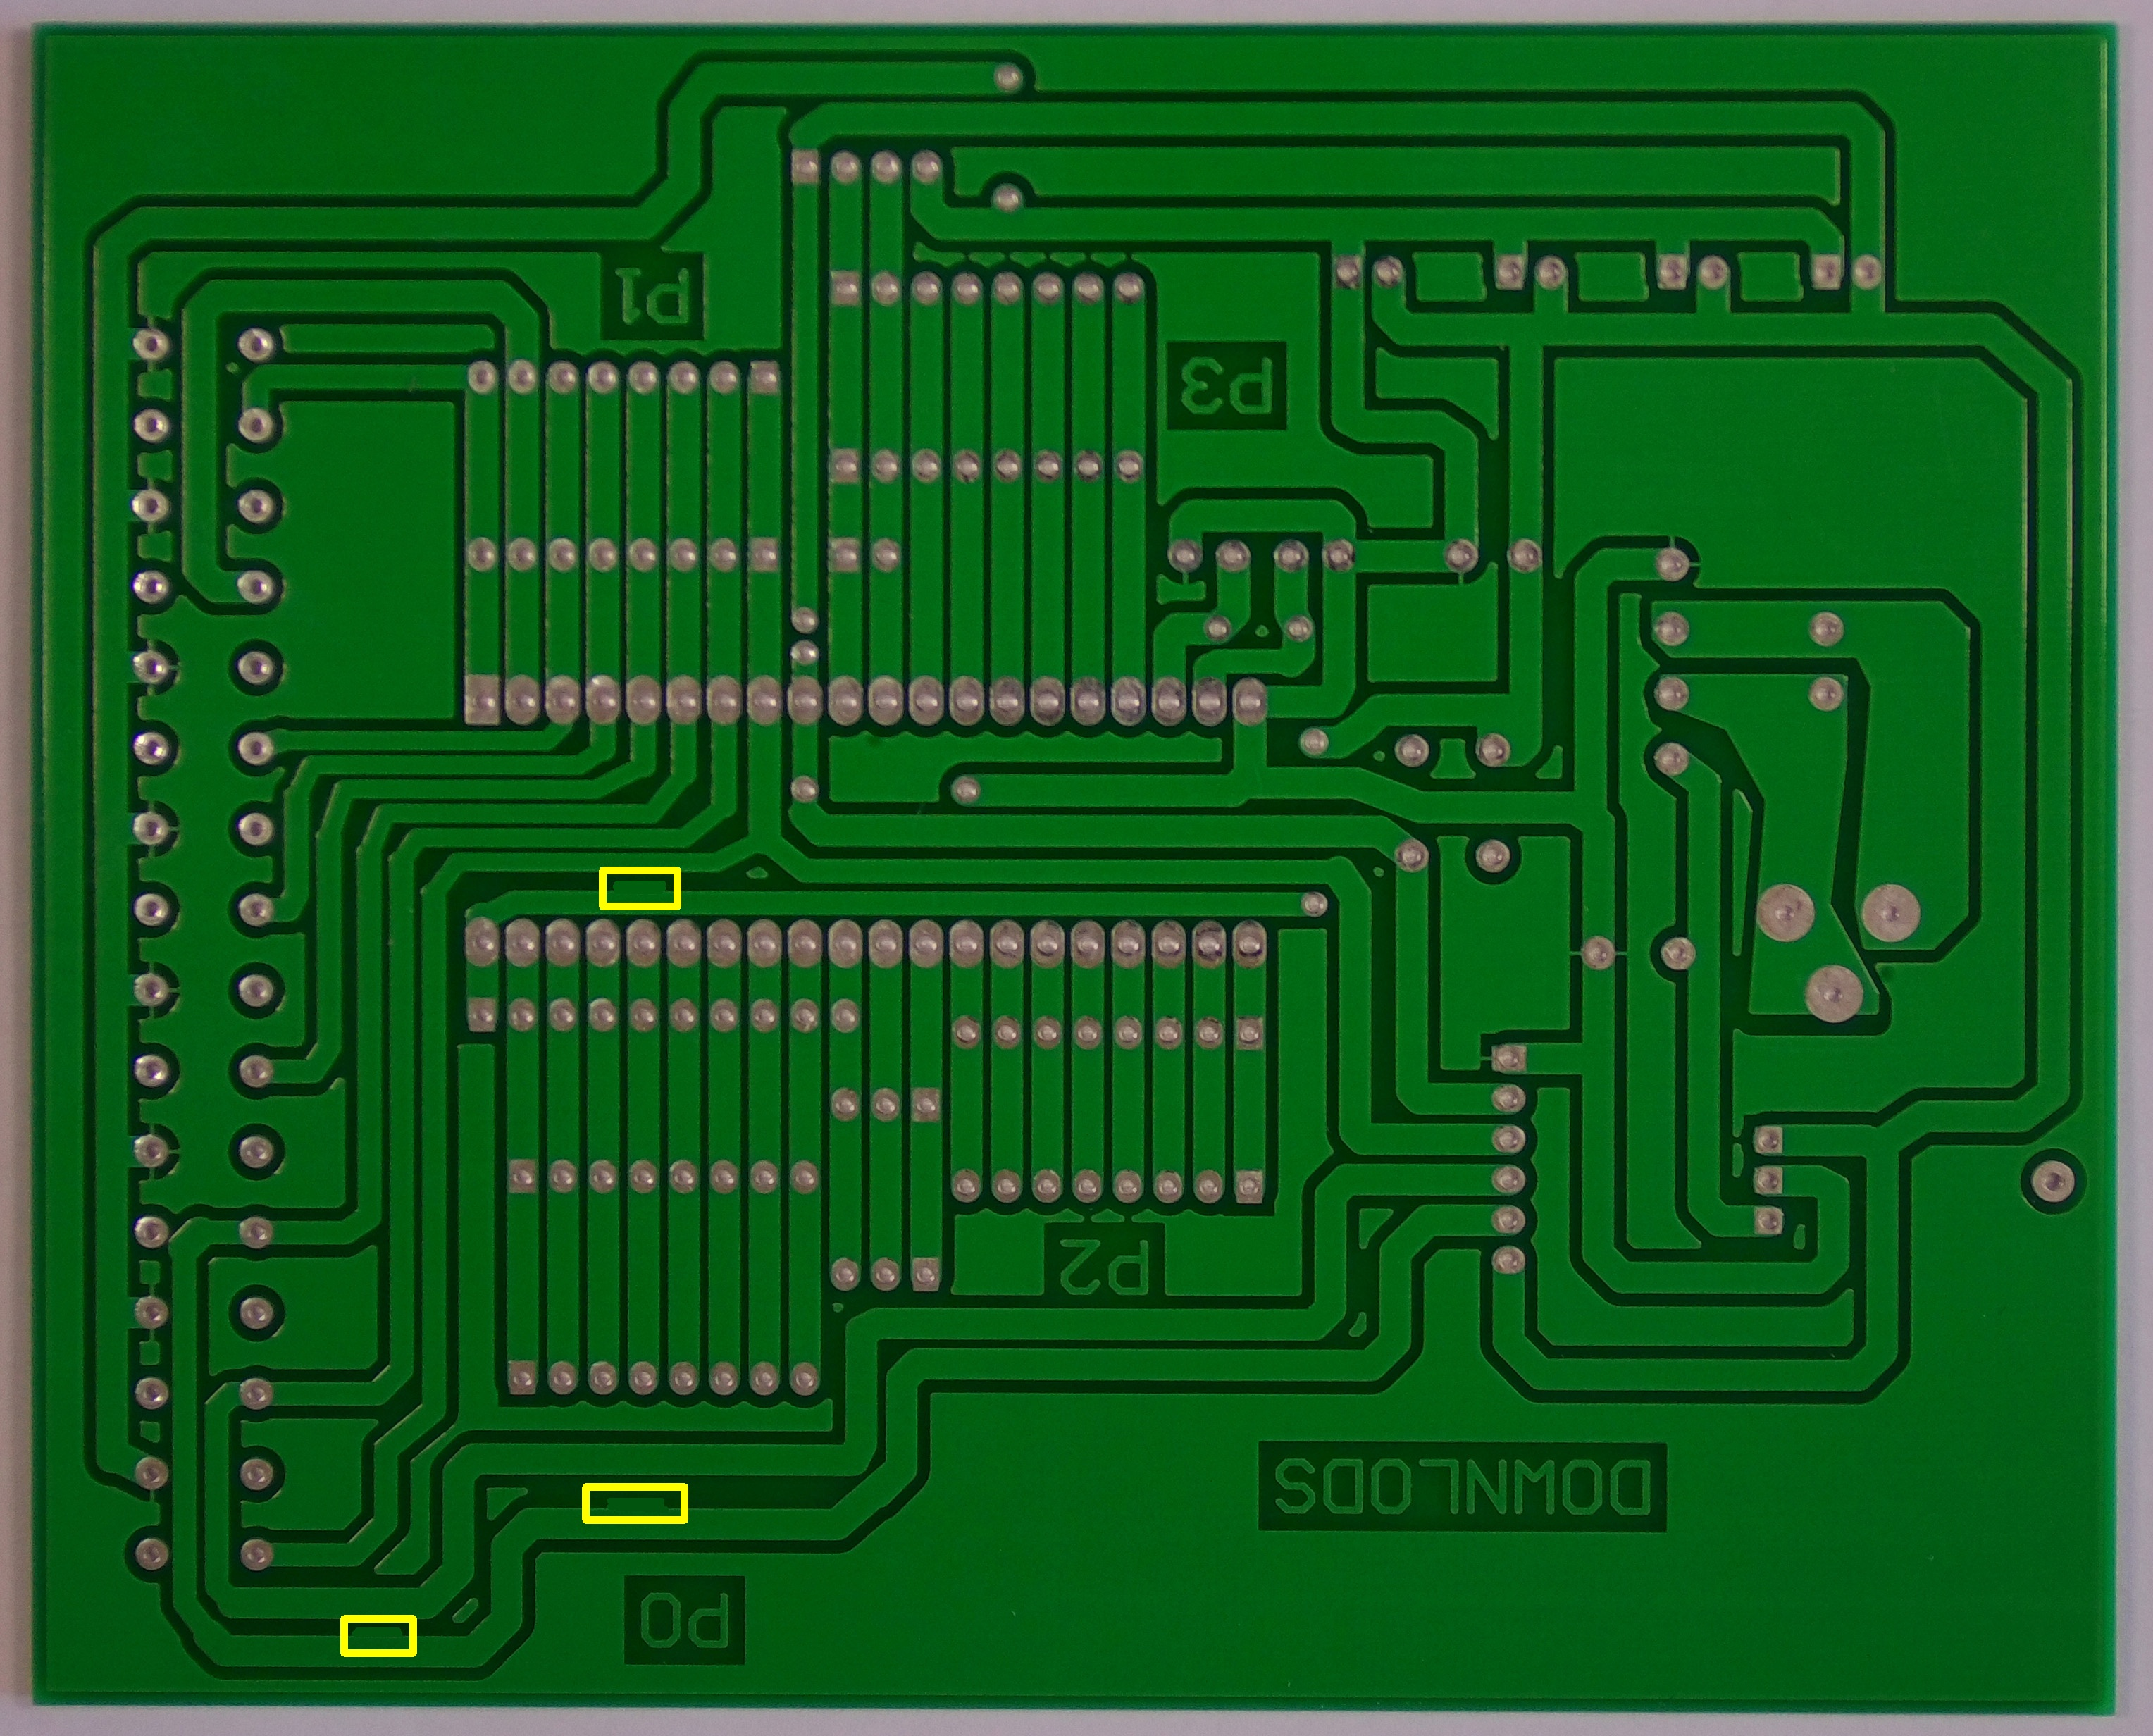}}
    \hfill
    \subfloat[Proposed Model: Open Circuit\label{6a}]{%
       \includegraphics[width=0.49\linewidth]{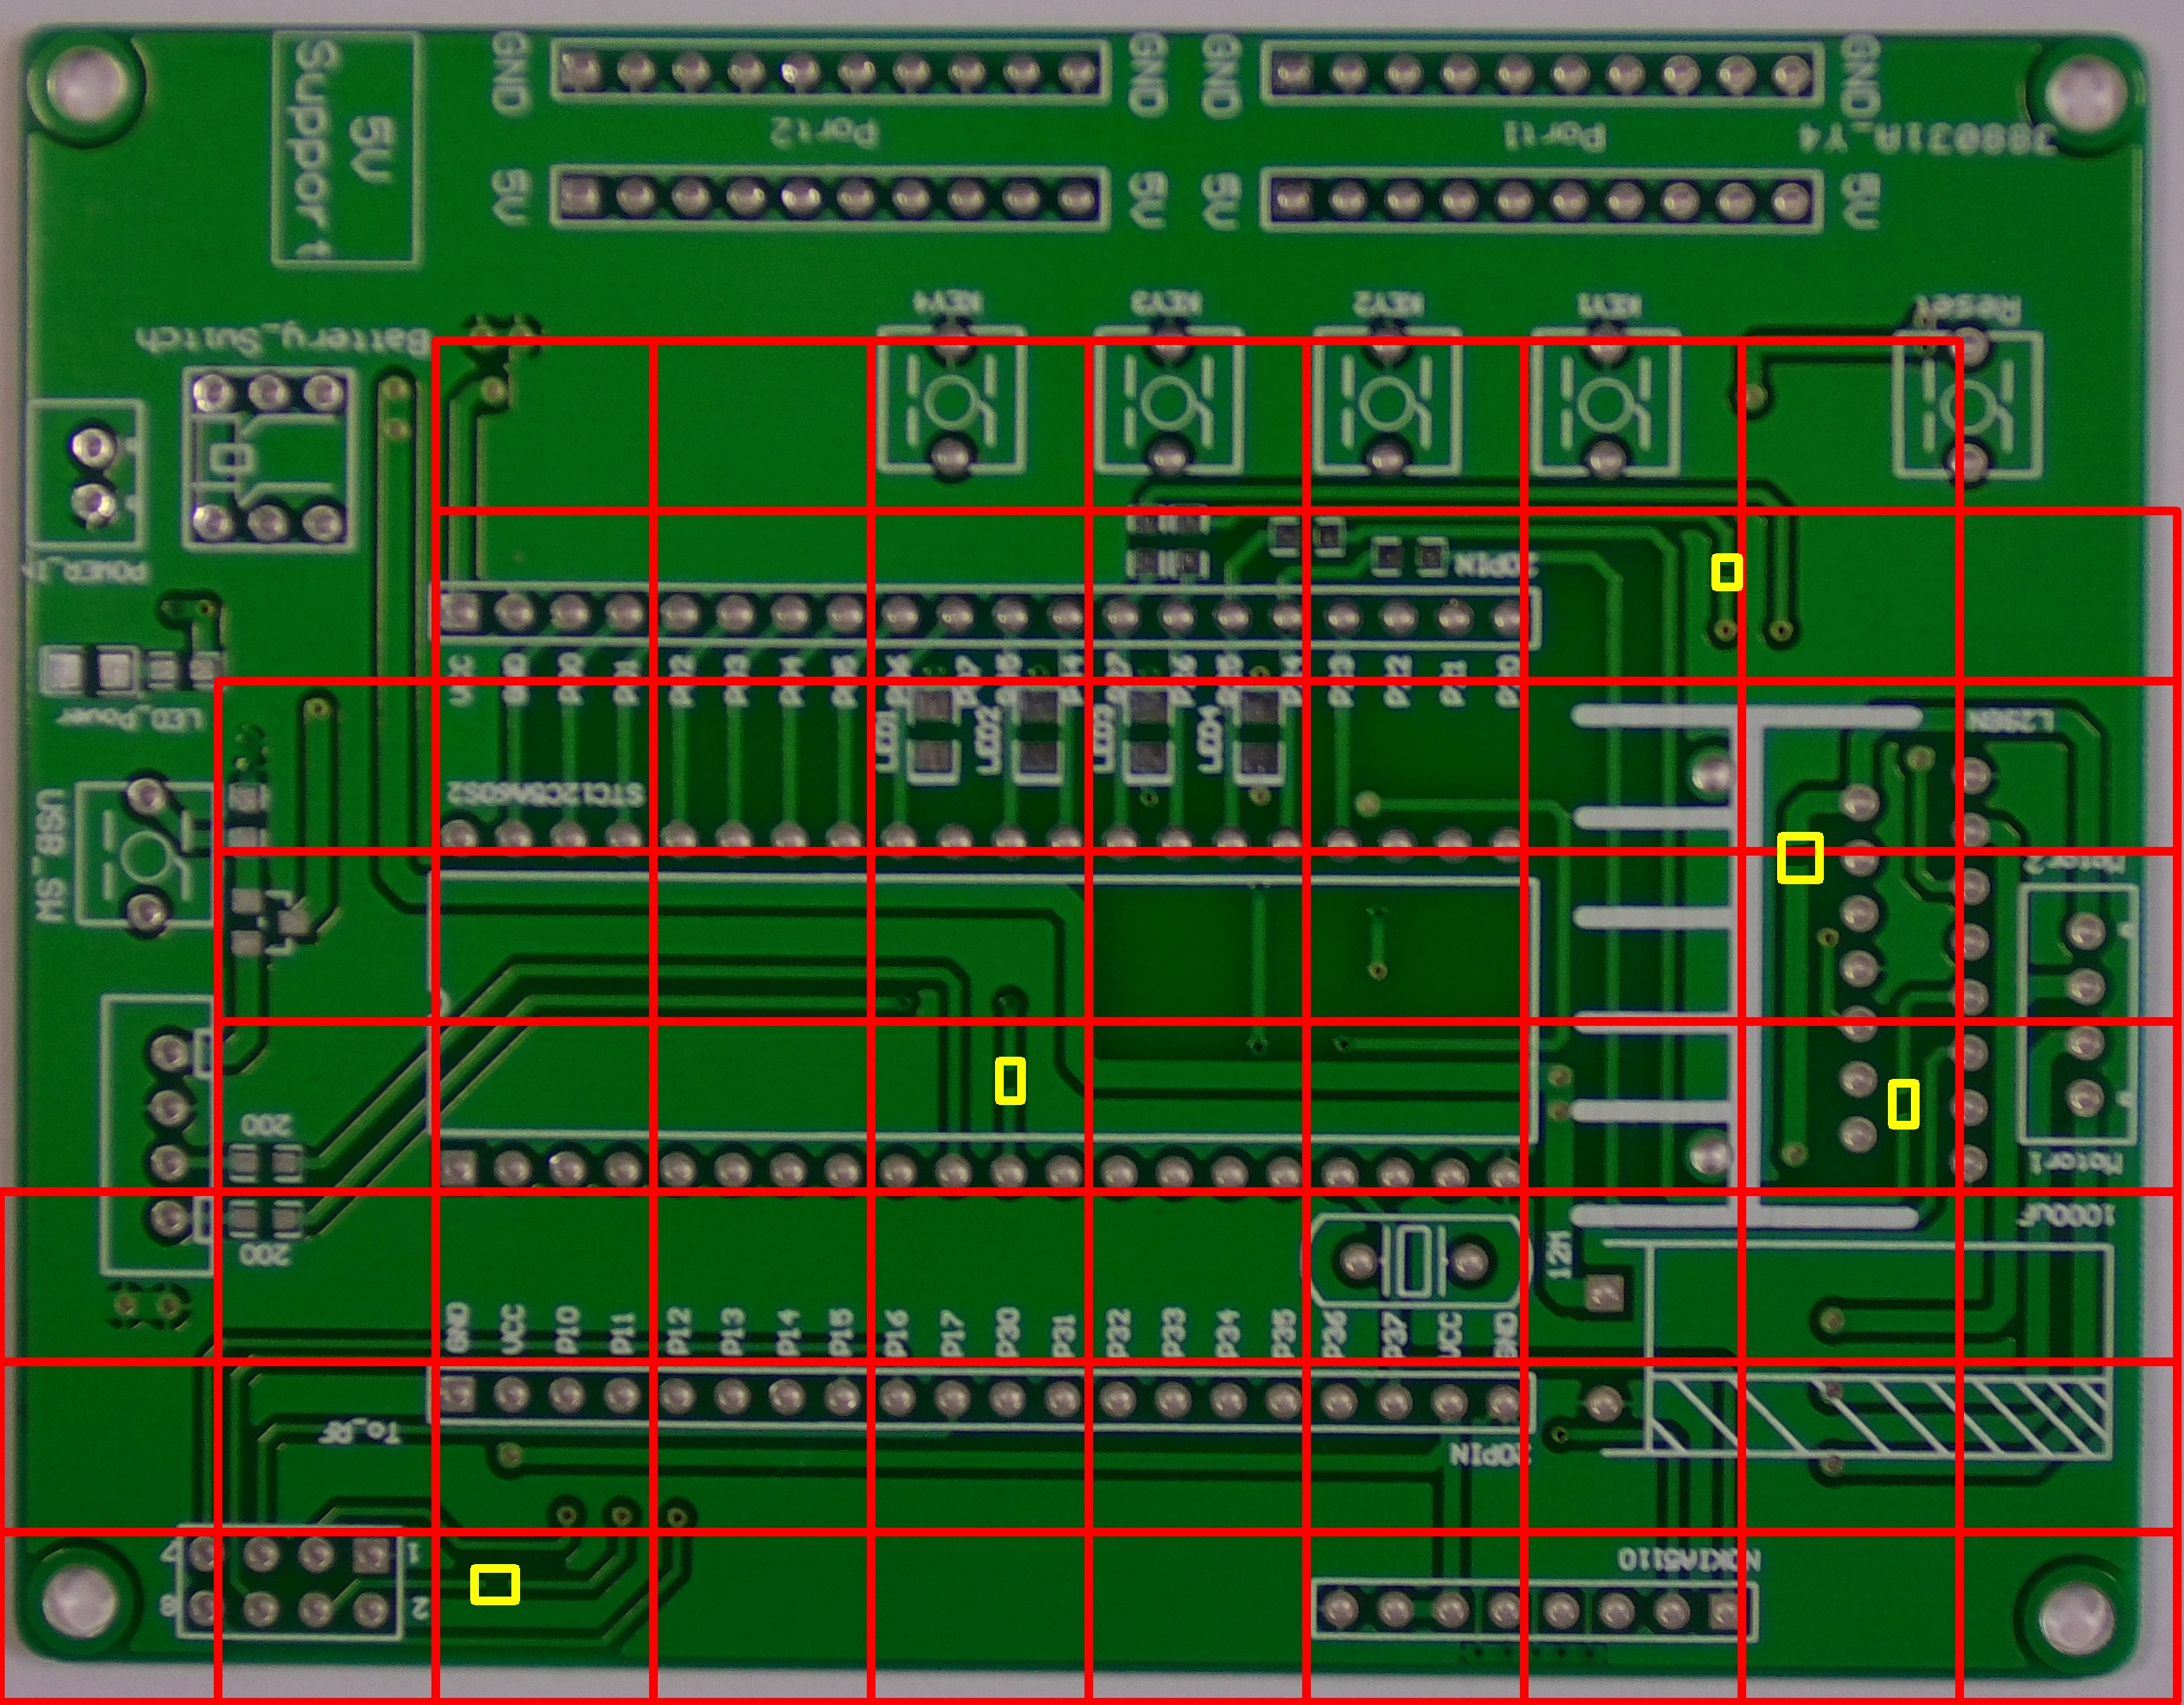}}
    \hfill
    \subfloat[Proposed Model: Spur\label{6b}]{%
       \includegraphics[width=0.48\linewidth]{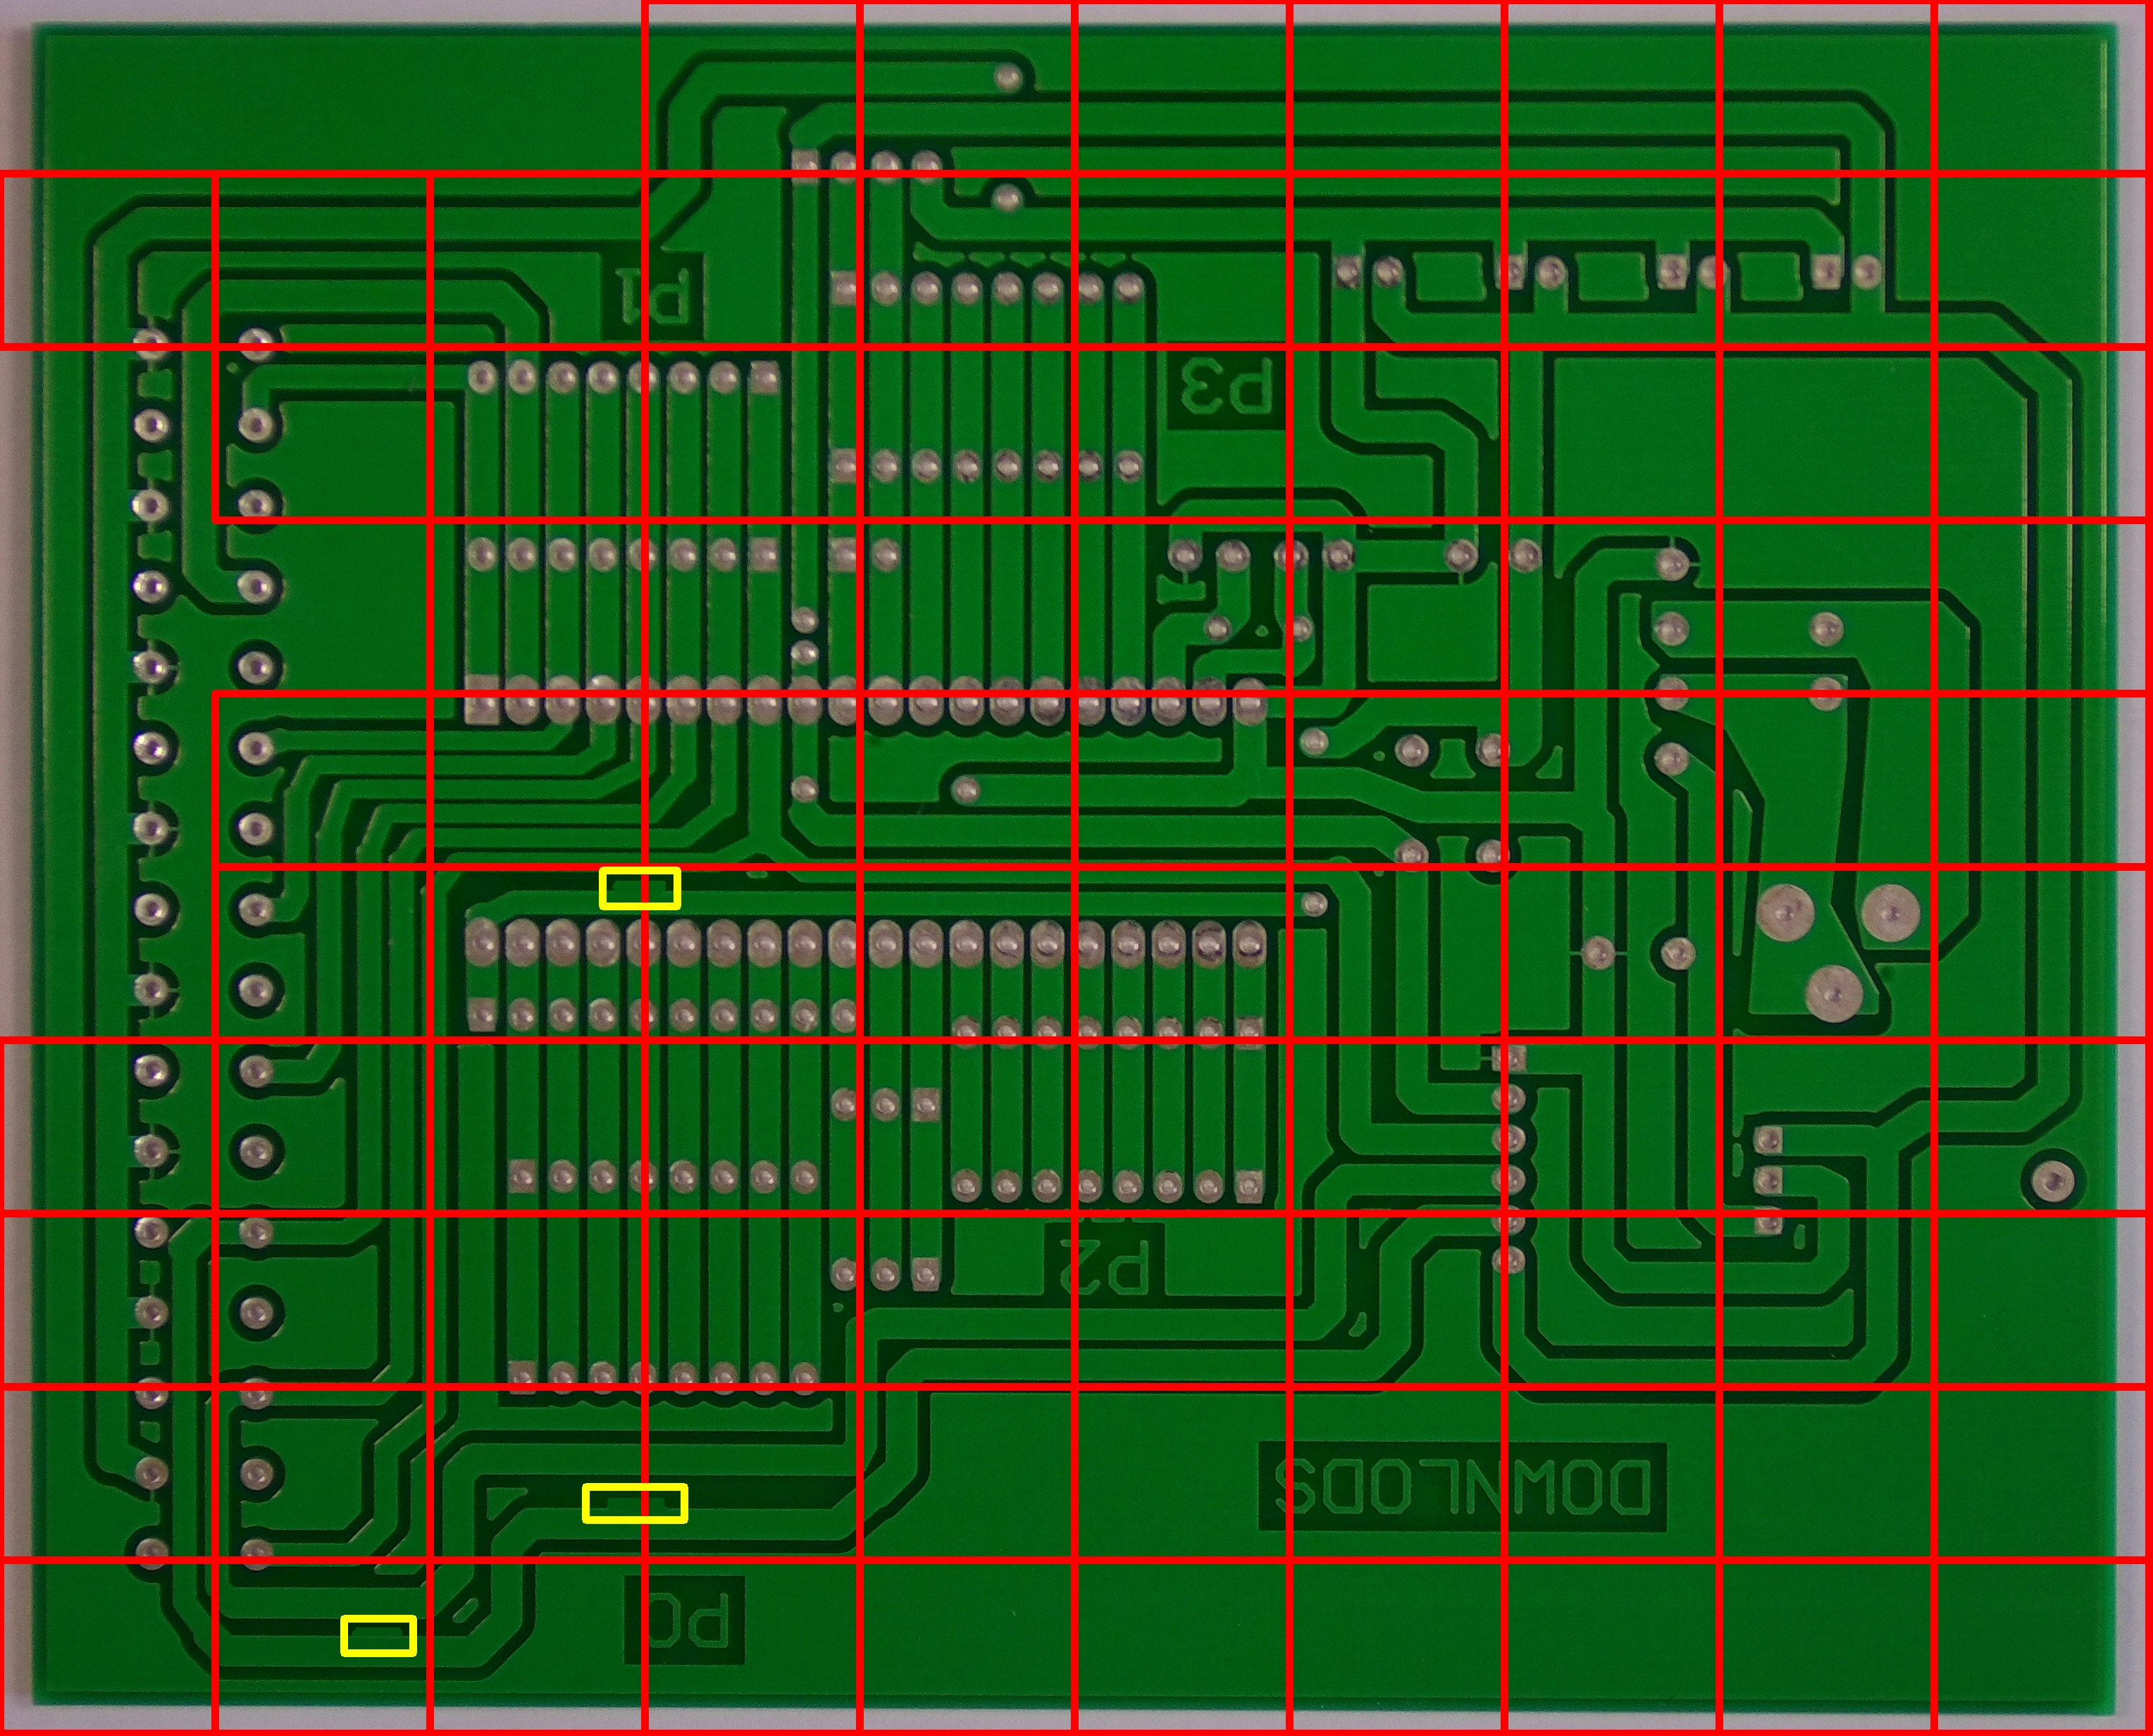}}
    \hfill
  \caption{Comparison of Pre-trained models vs Our Non pre-trained model}
  \label{fig:detection_results_TL}
\end{figure}

%Defect detection benchmark
\begin{figure}[h!] 
    \centering
  \subfloat[Open Circuit\label{6i}]{%
        \includegraphics[width=0.49\linewidth]{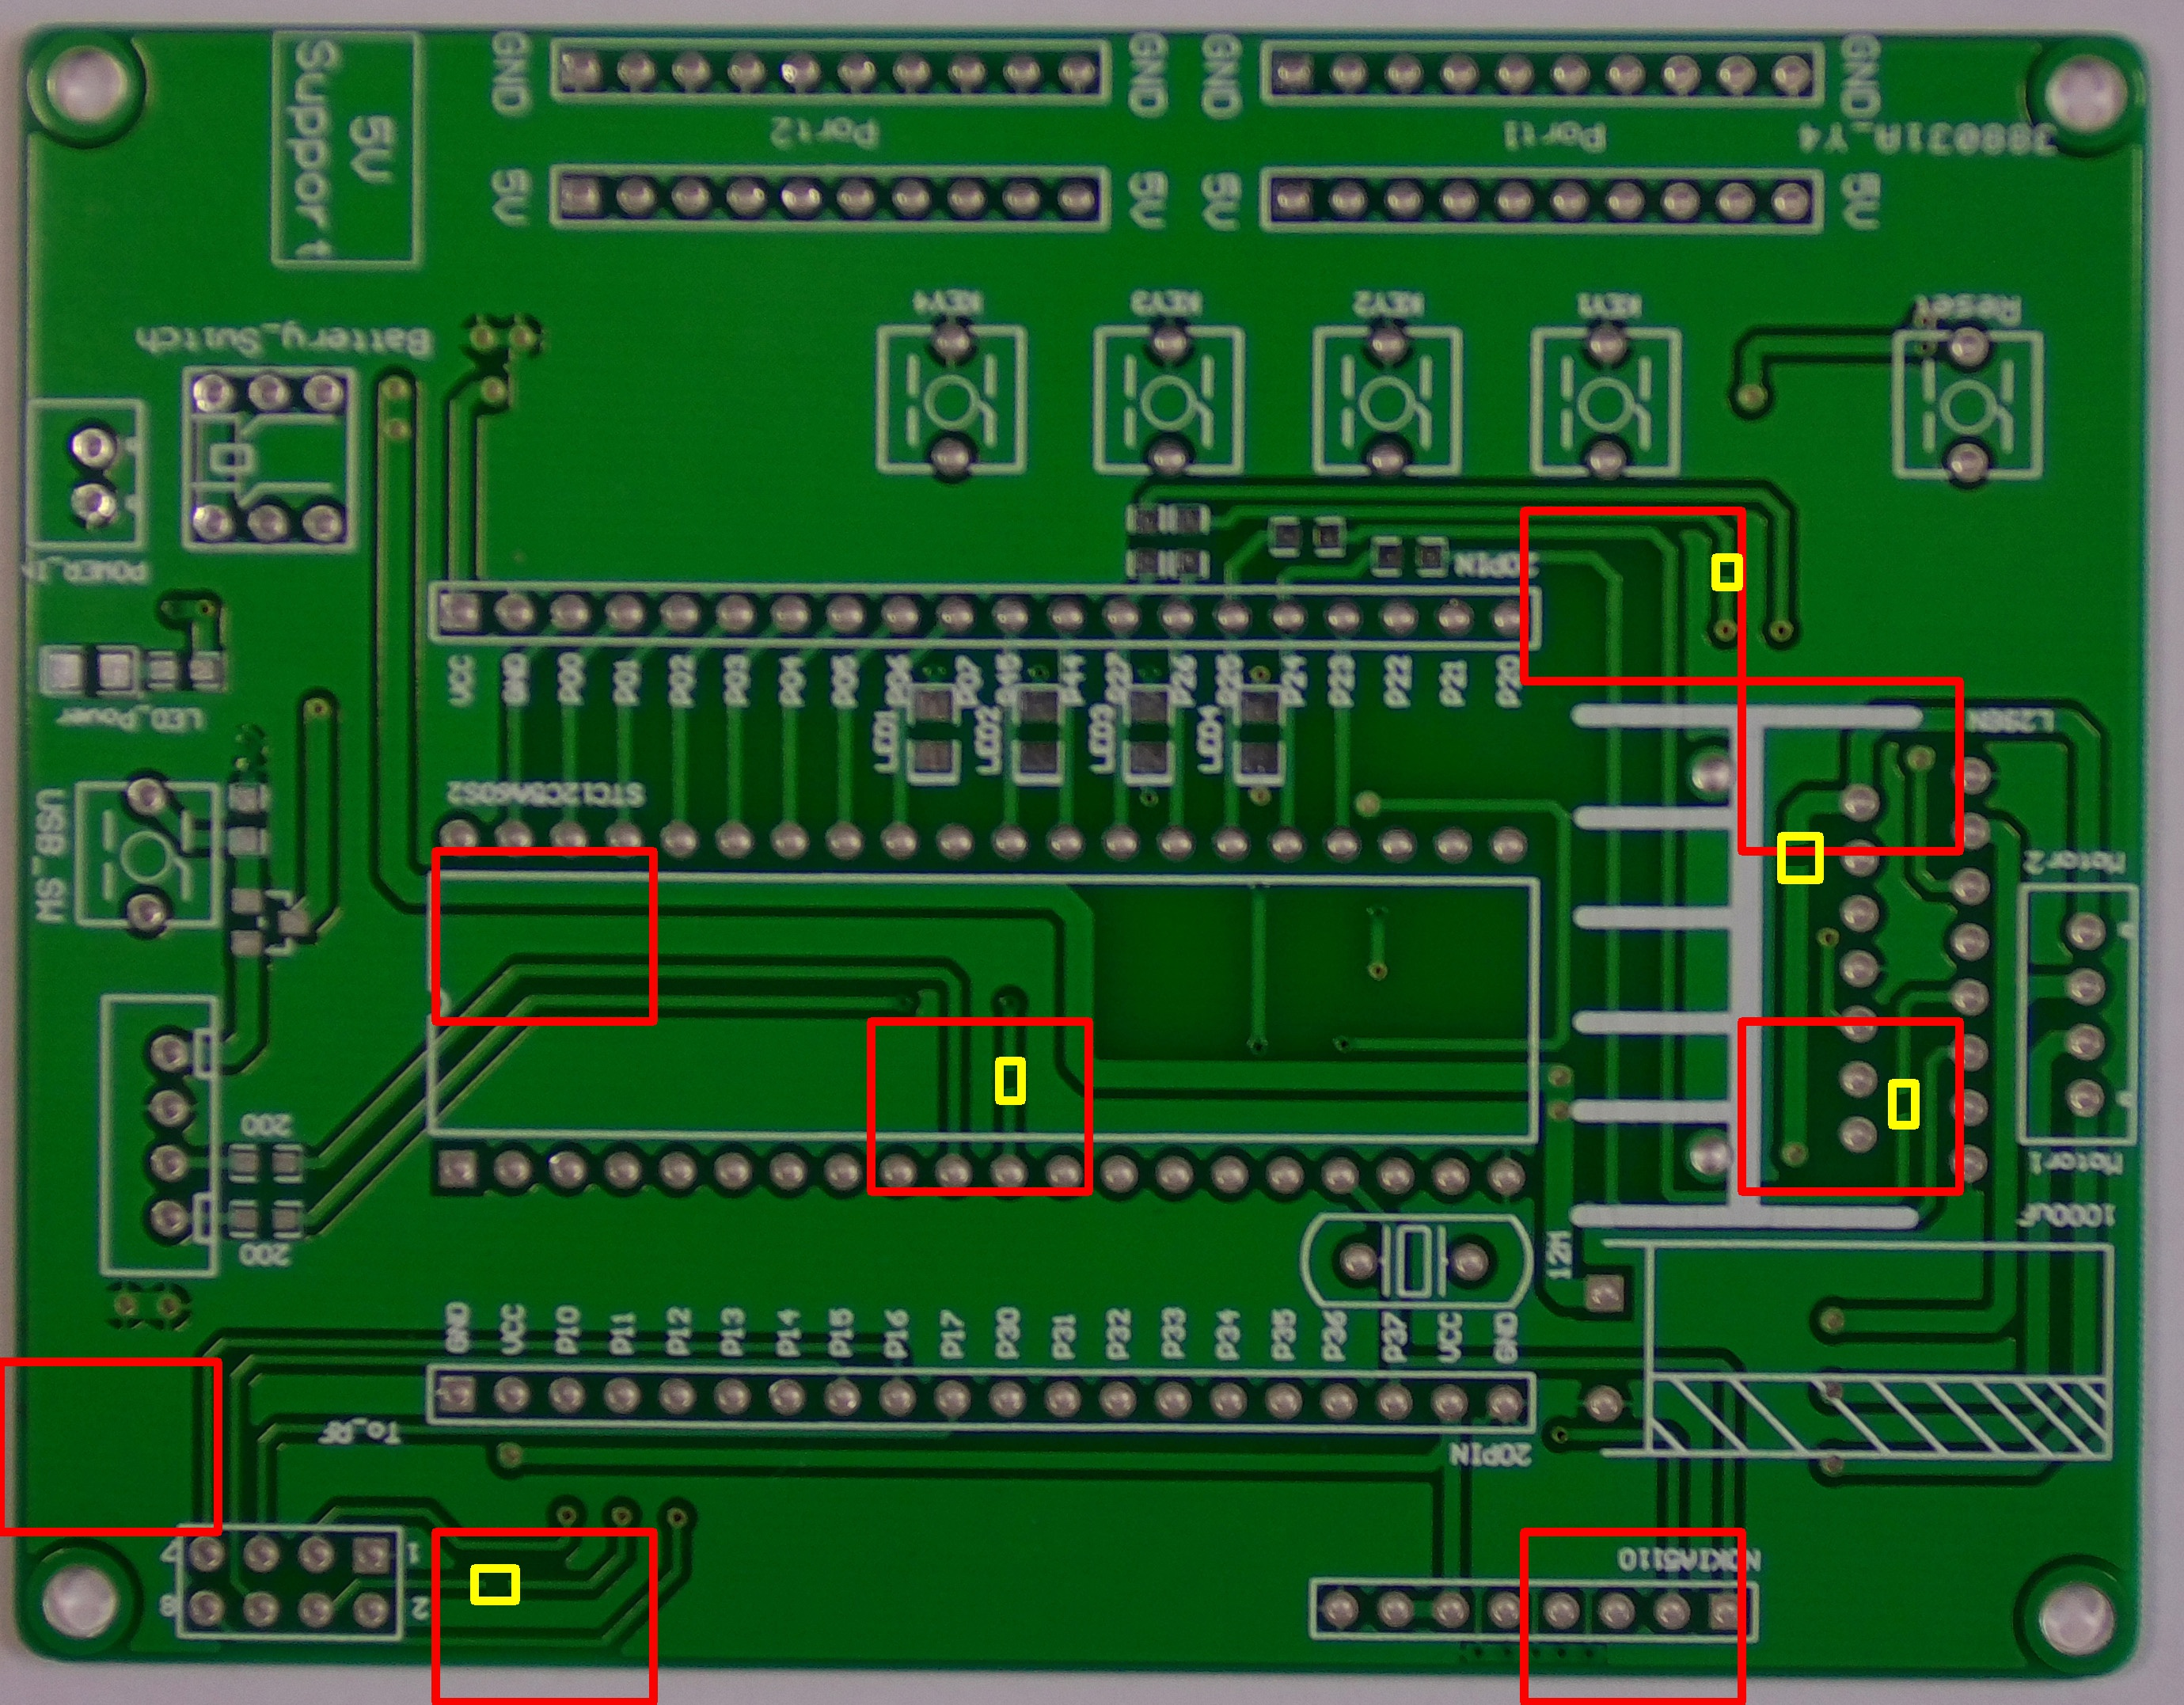}}
     \hfill
     \subfloat[Spur\label{6j}]{%
        \includegraphics[width=0.48\linewidth]{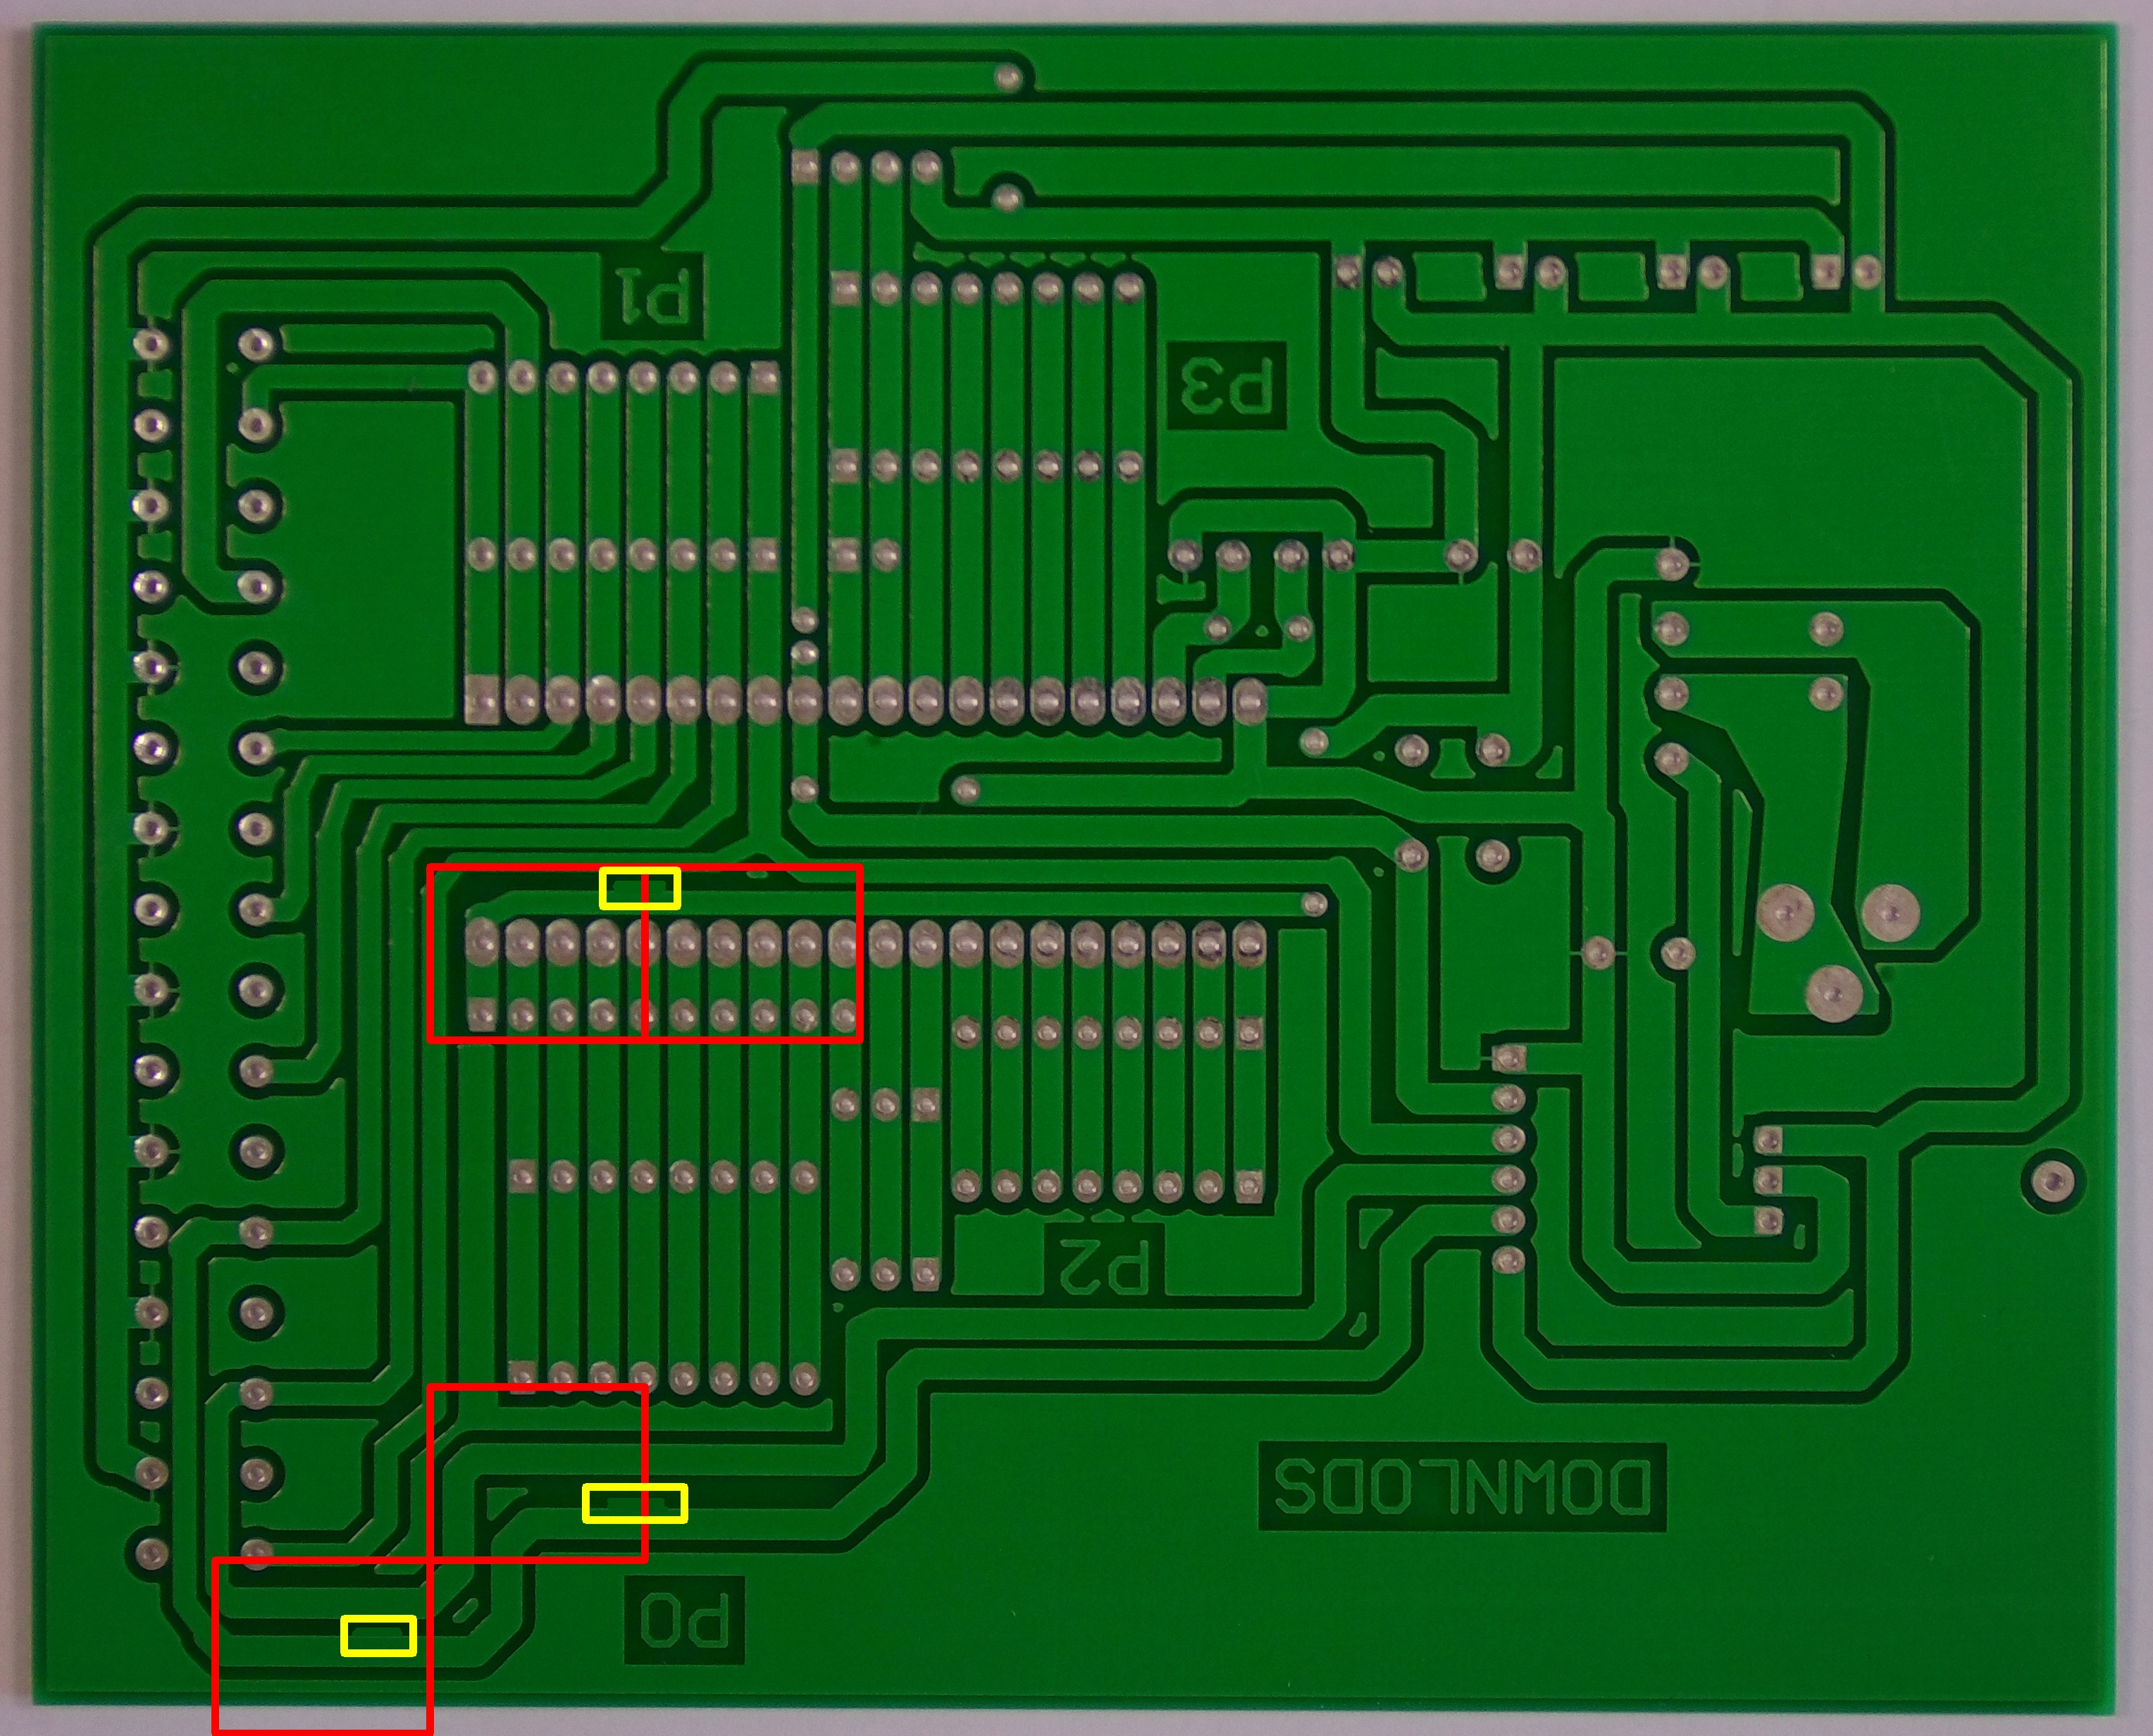}}
     \hfill
  \caption{Benchmark result with Xception (pre-trained on ImageNet) implemented on desktop}
  \label{fig:detection_results_benchmark}
\end{figure}

%Defect detection without pre-training
\begin{figure}[h!] 
    \centering
  \subfloat[Proposed Model: Open Circuit\label{6a}]{%
       \includegraphics[width=0.49\linewidth]{Contents/figures/inf_opencirc_xlite.jpg}}
    \hfill
    \subfloat[Proposed Model: Spur\label{6b}]{%
       \includegraphics[width=0.48\linewidth]{Contents/figures/inf_spur_xlite.jpg}}
    \hfill
      
  \subfloat[EfficientNetV2B0: Open Circuit\label{6e}]{%
        \includegraphics[width=0.49\linewidth]{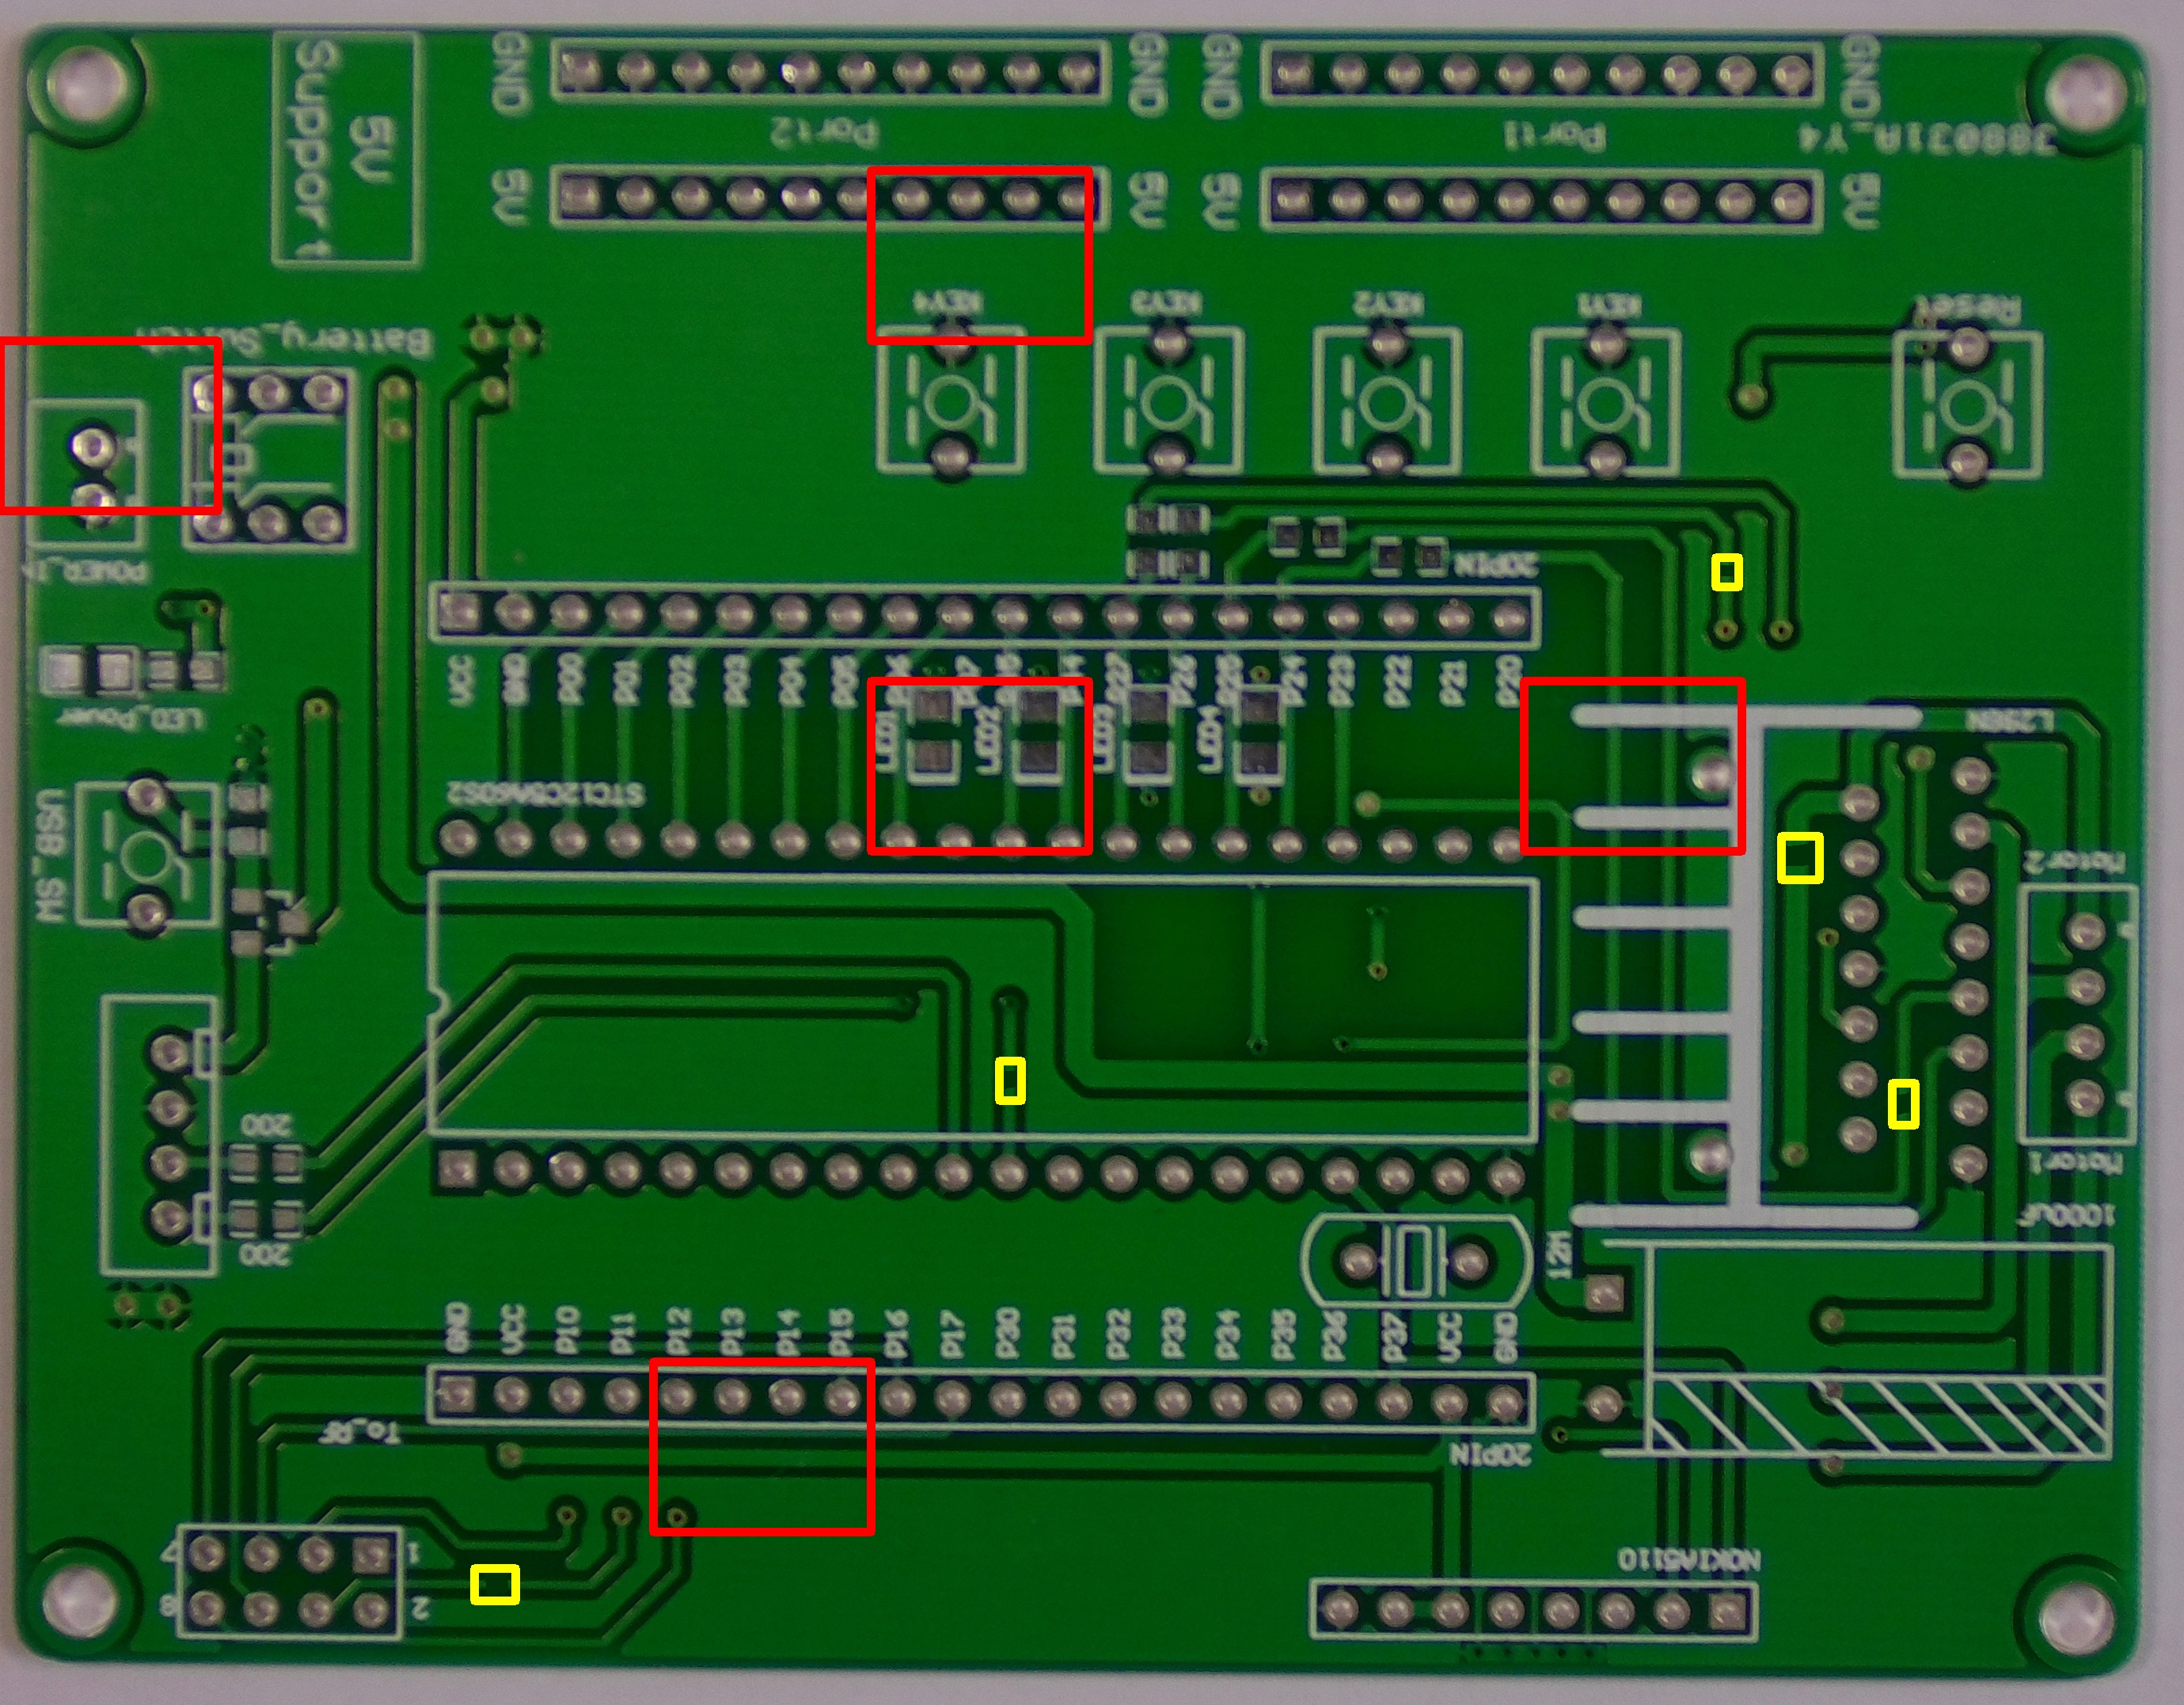}}
    \hfill
    \subfloat[EfficientNetV2B0: Spur\label{6f}]{%
        \includegraphics[width=0.48\linewidth]{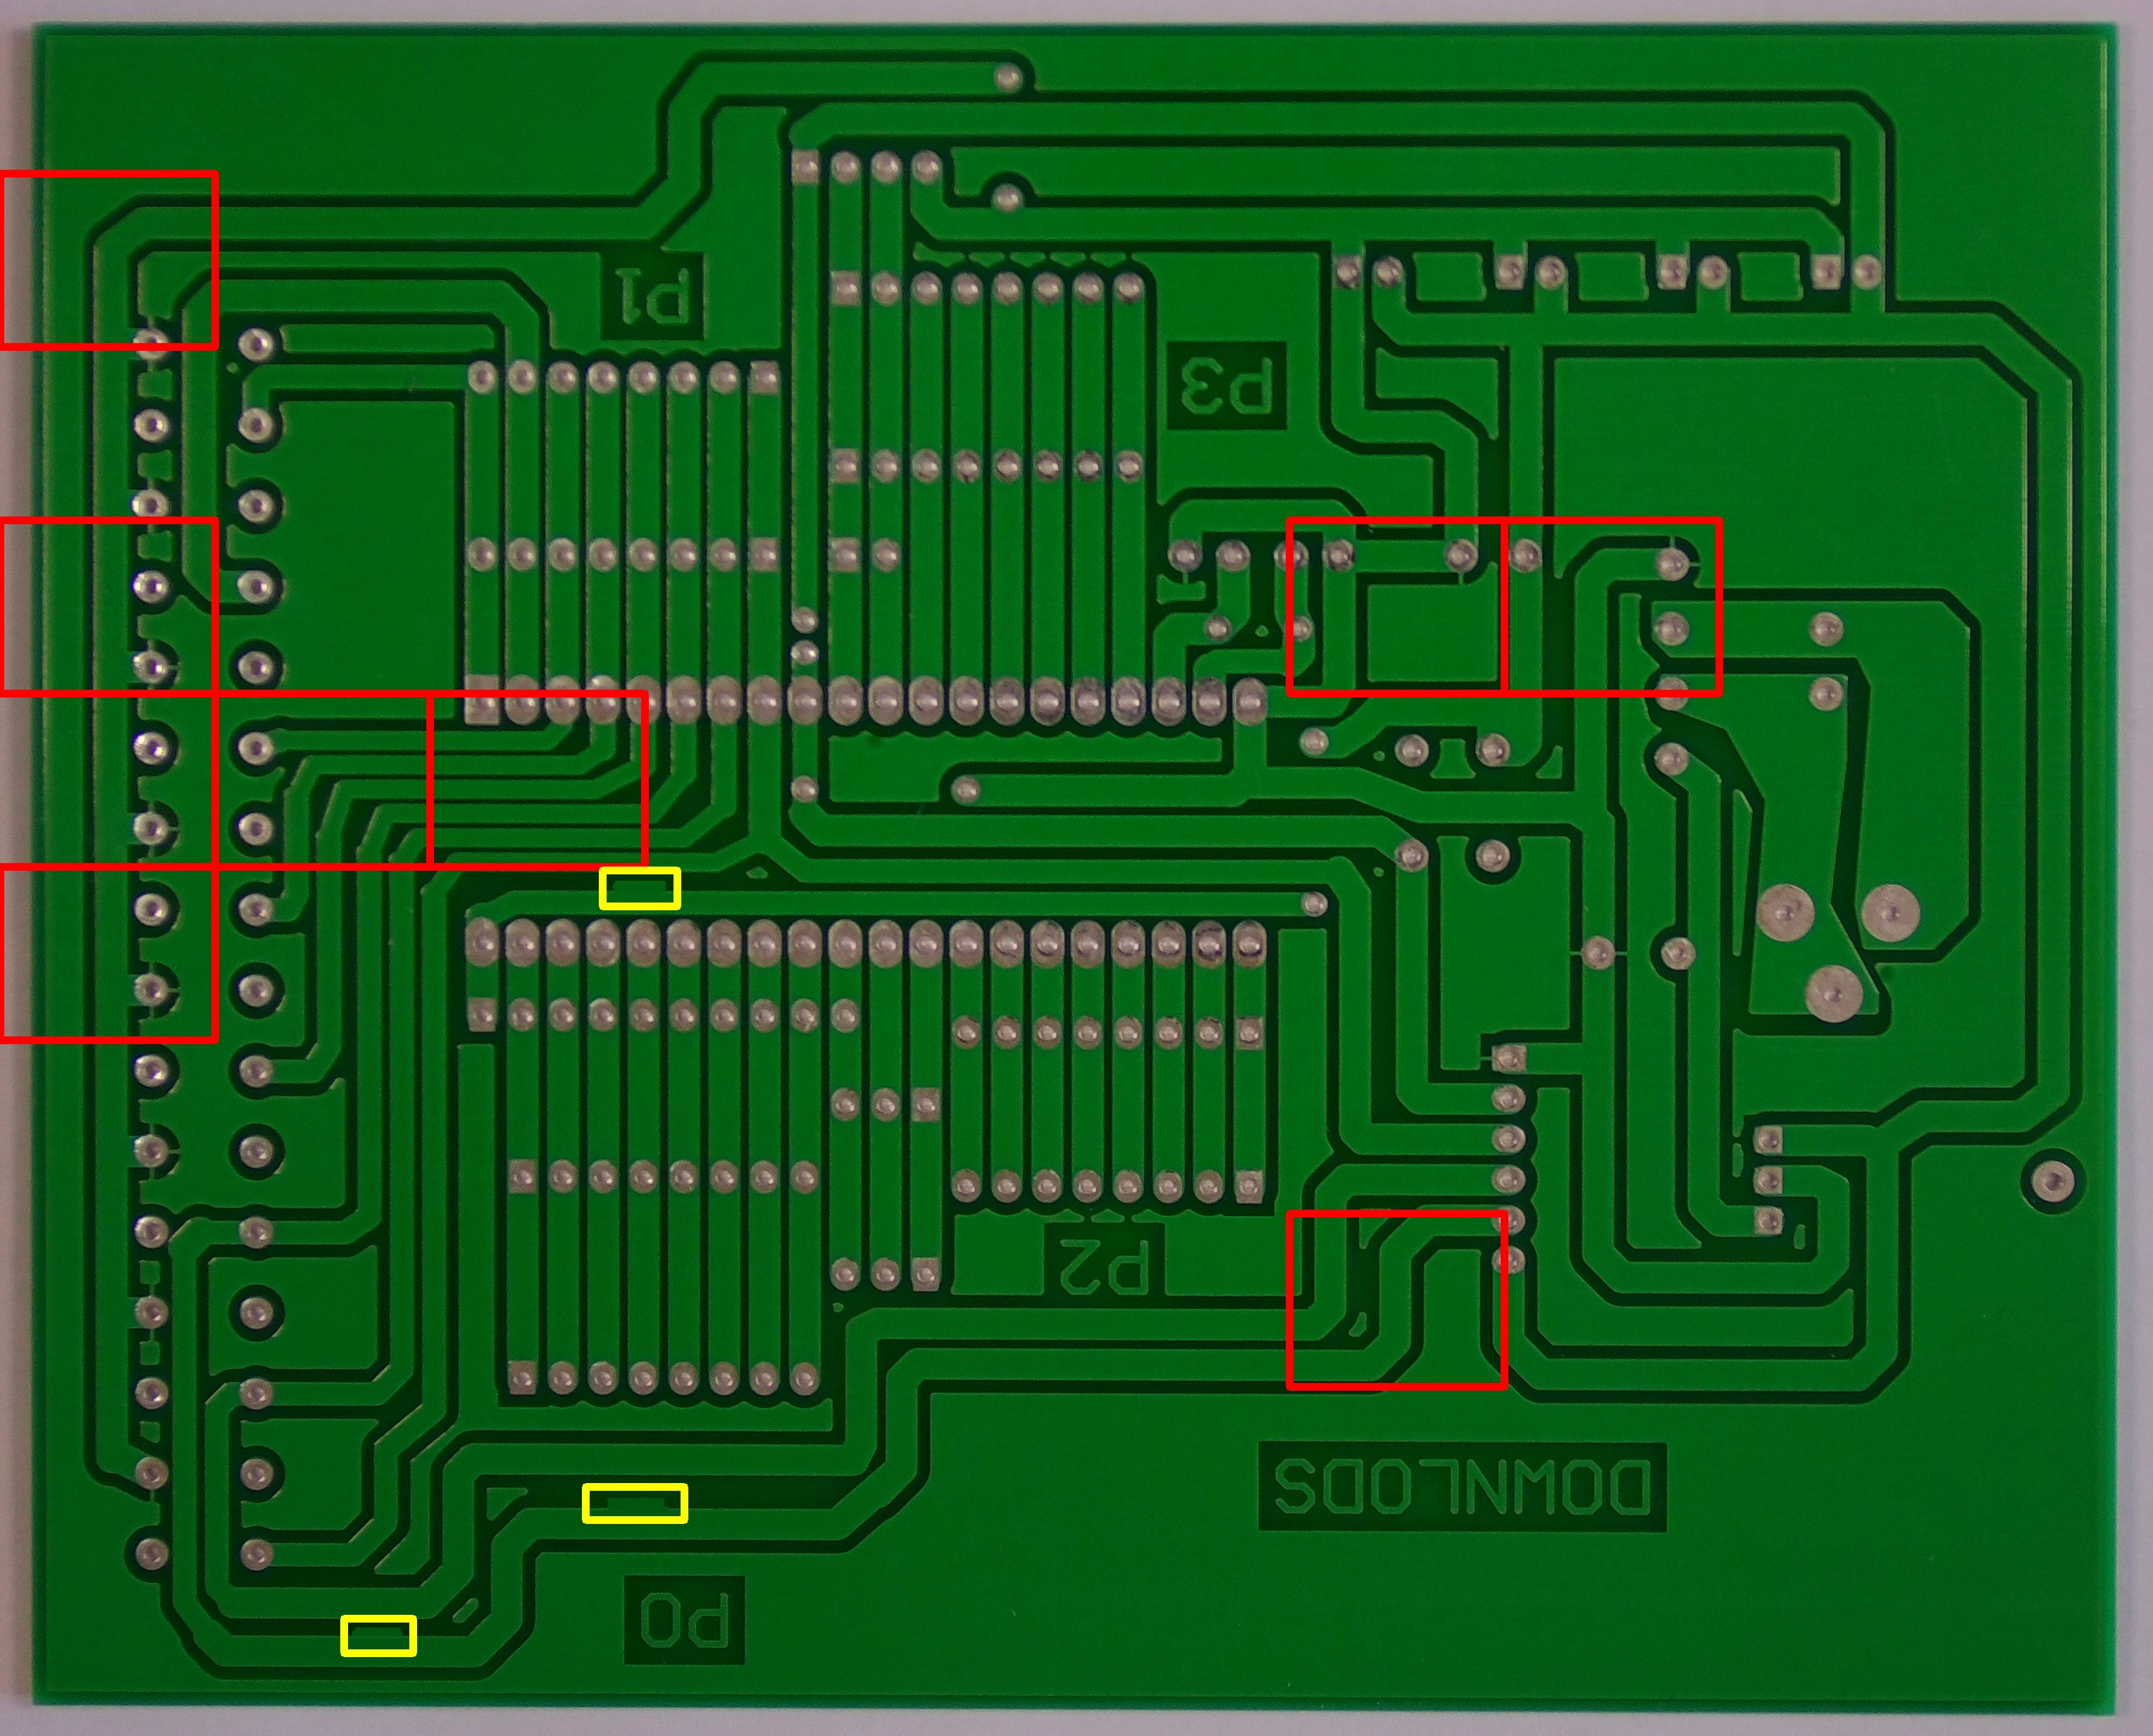}}
    \hfill
    
  \subfloat[MobileNetV2: Open Circuit\label{6c}]{%
        \includegraphics[width=0.49\linewidth]{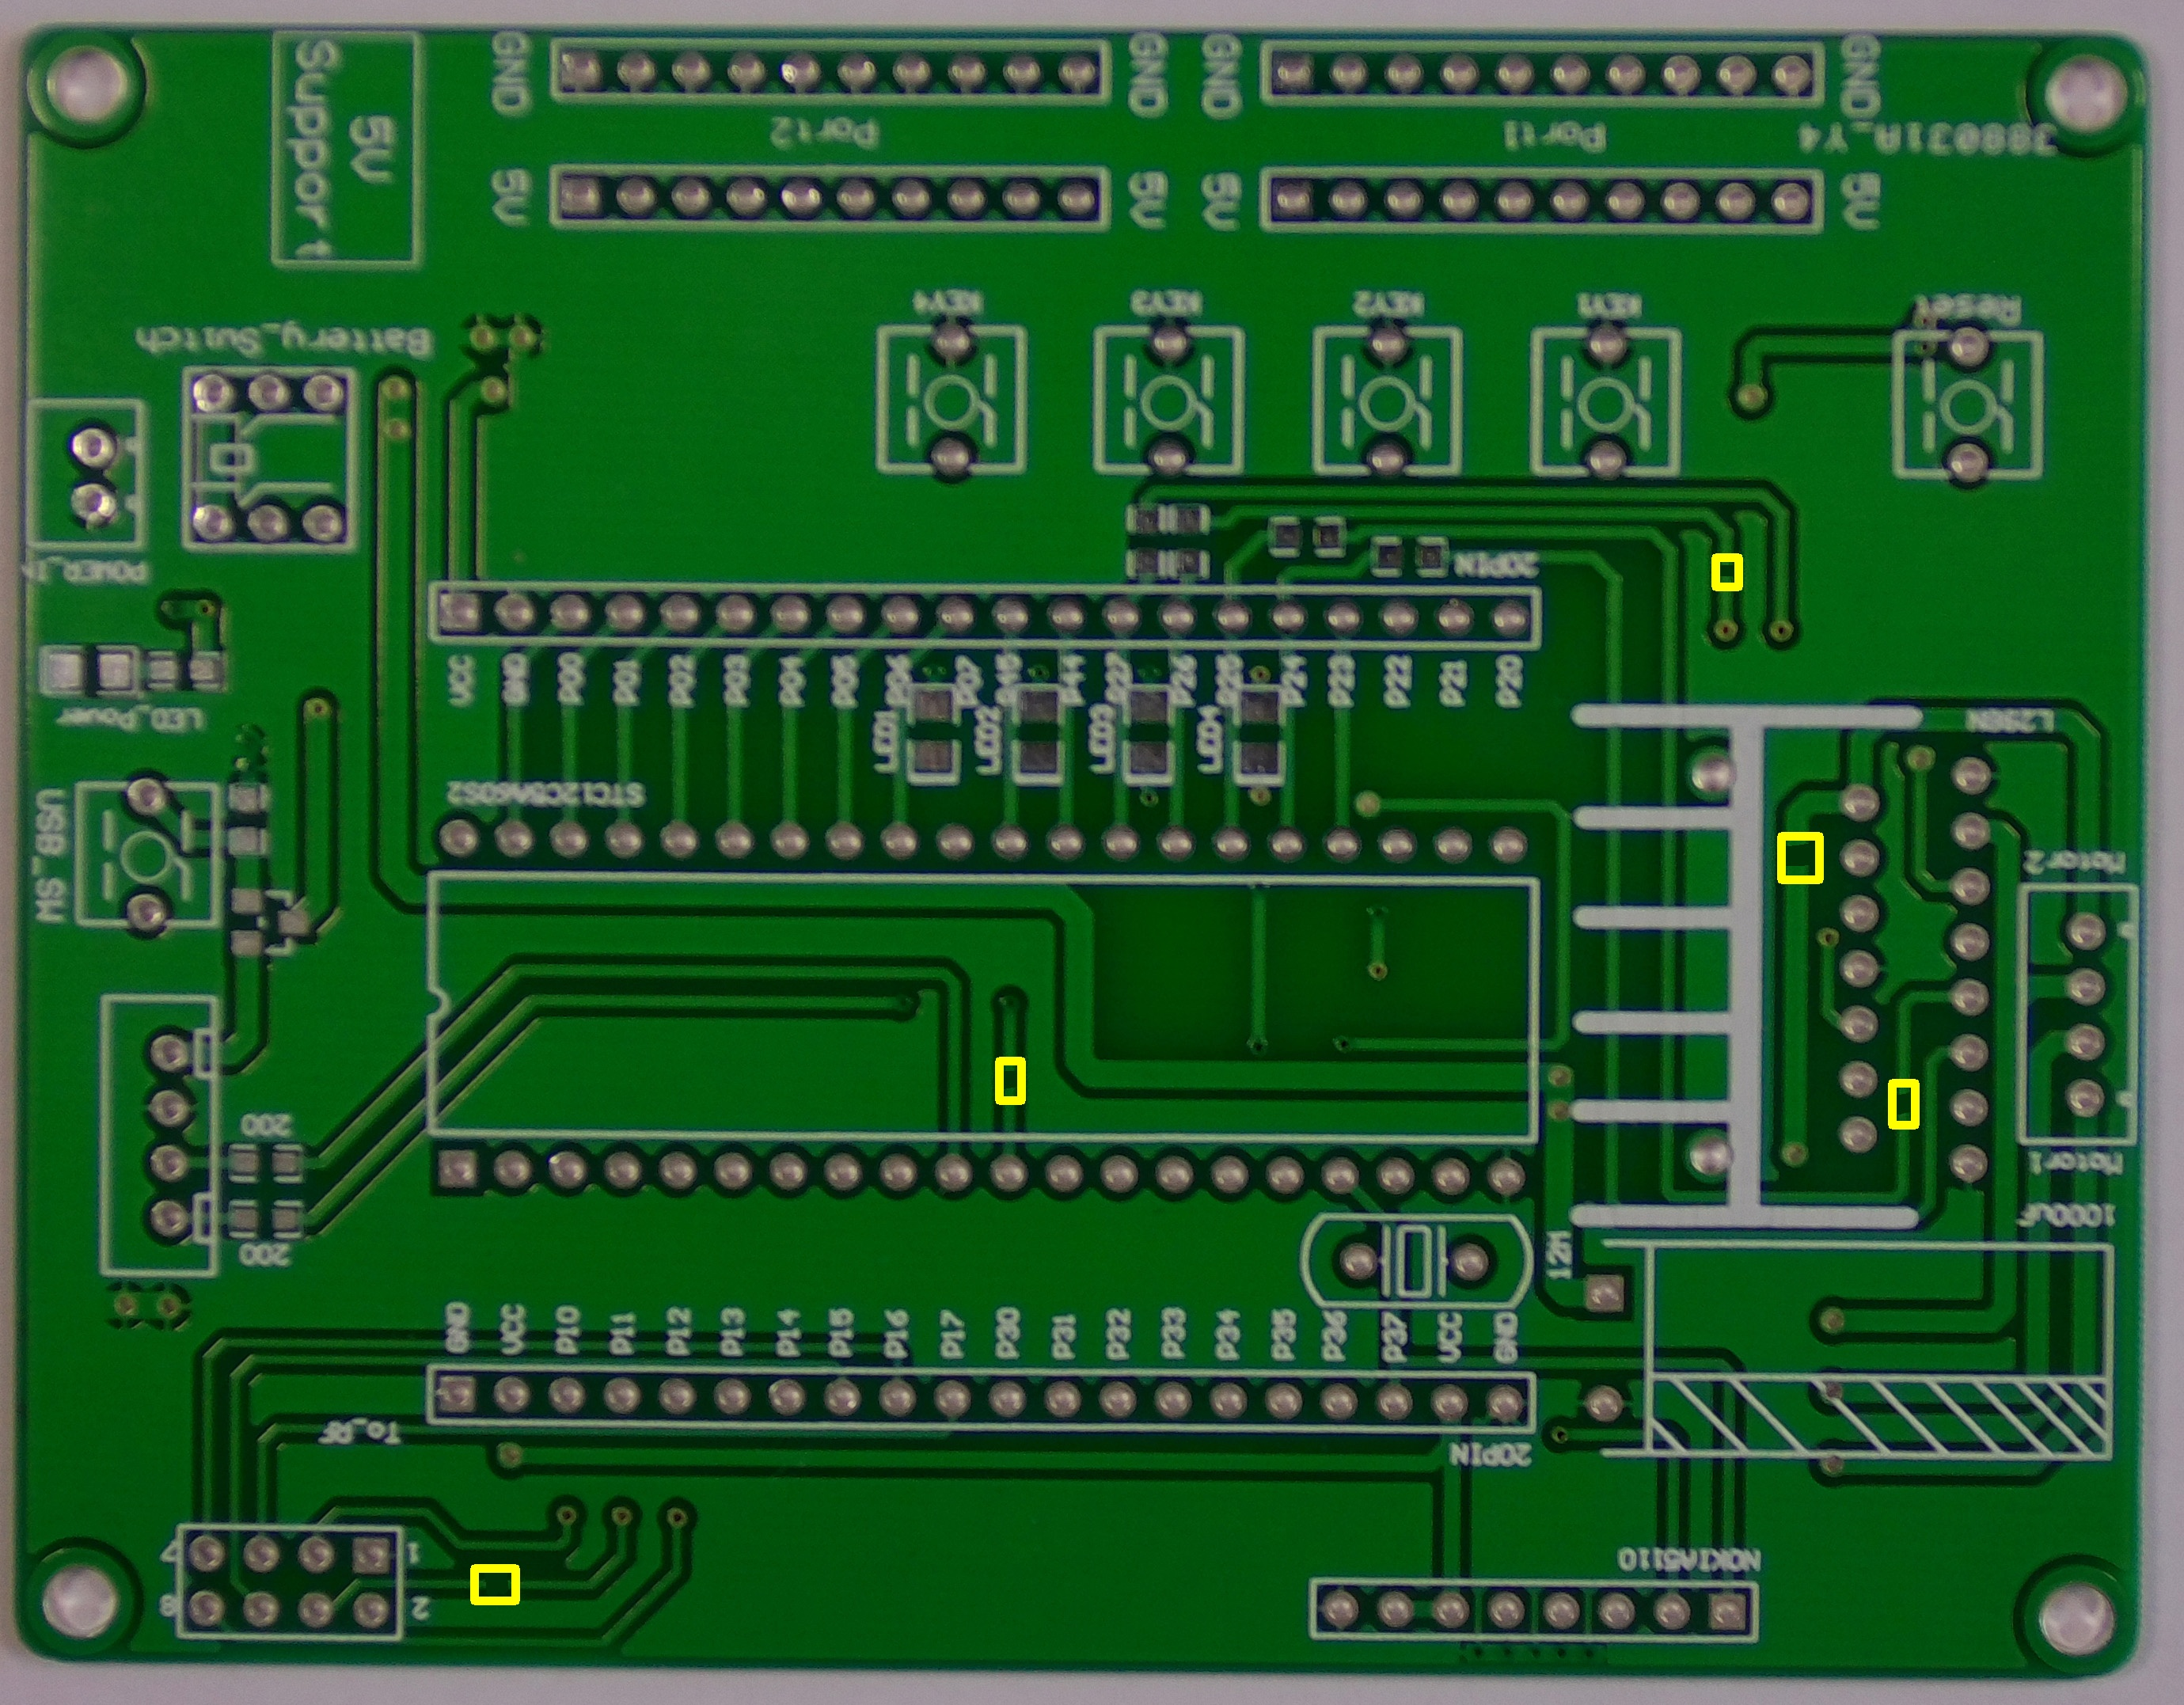}}
    \hfill
    \subfloat[MobileNetV2: Spur\label{6d}]{%
        \includegraphics[width=0.48\linewidth]{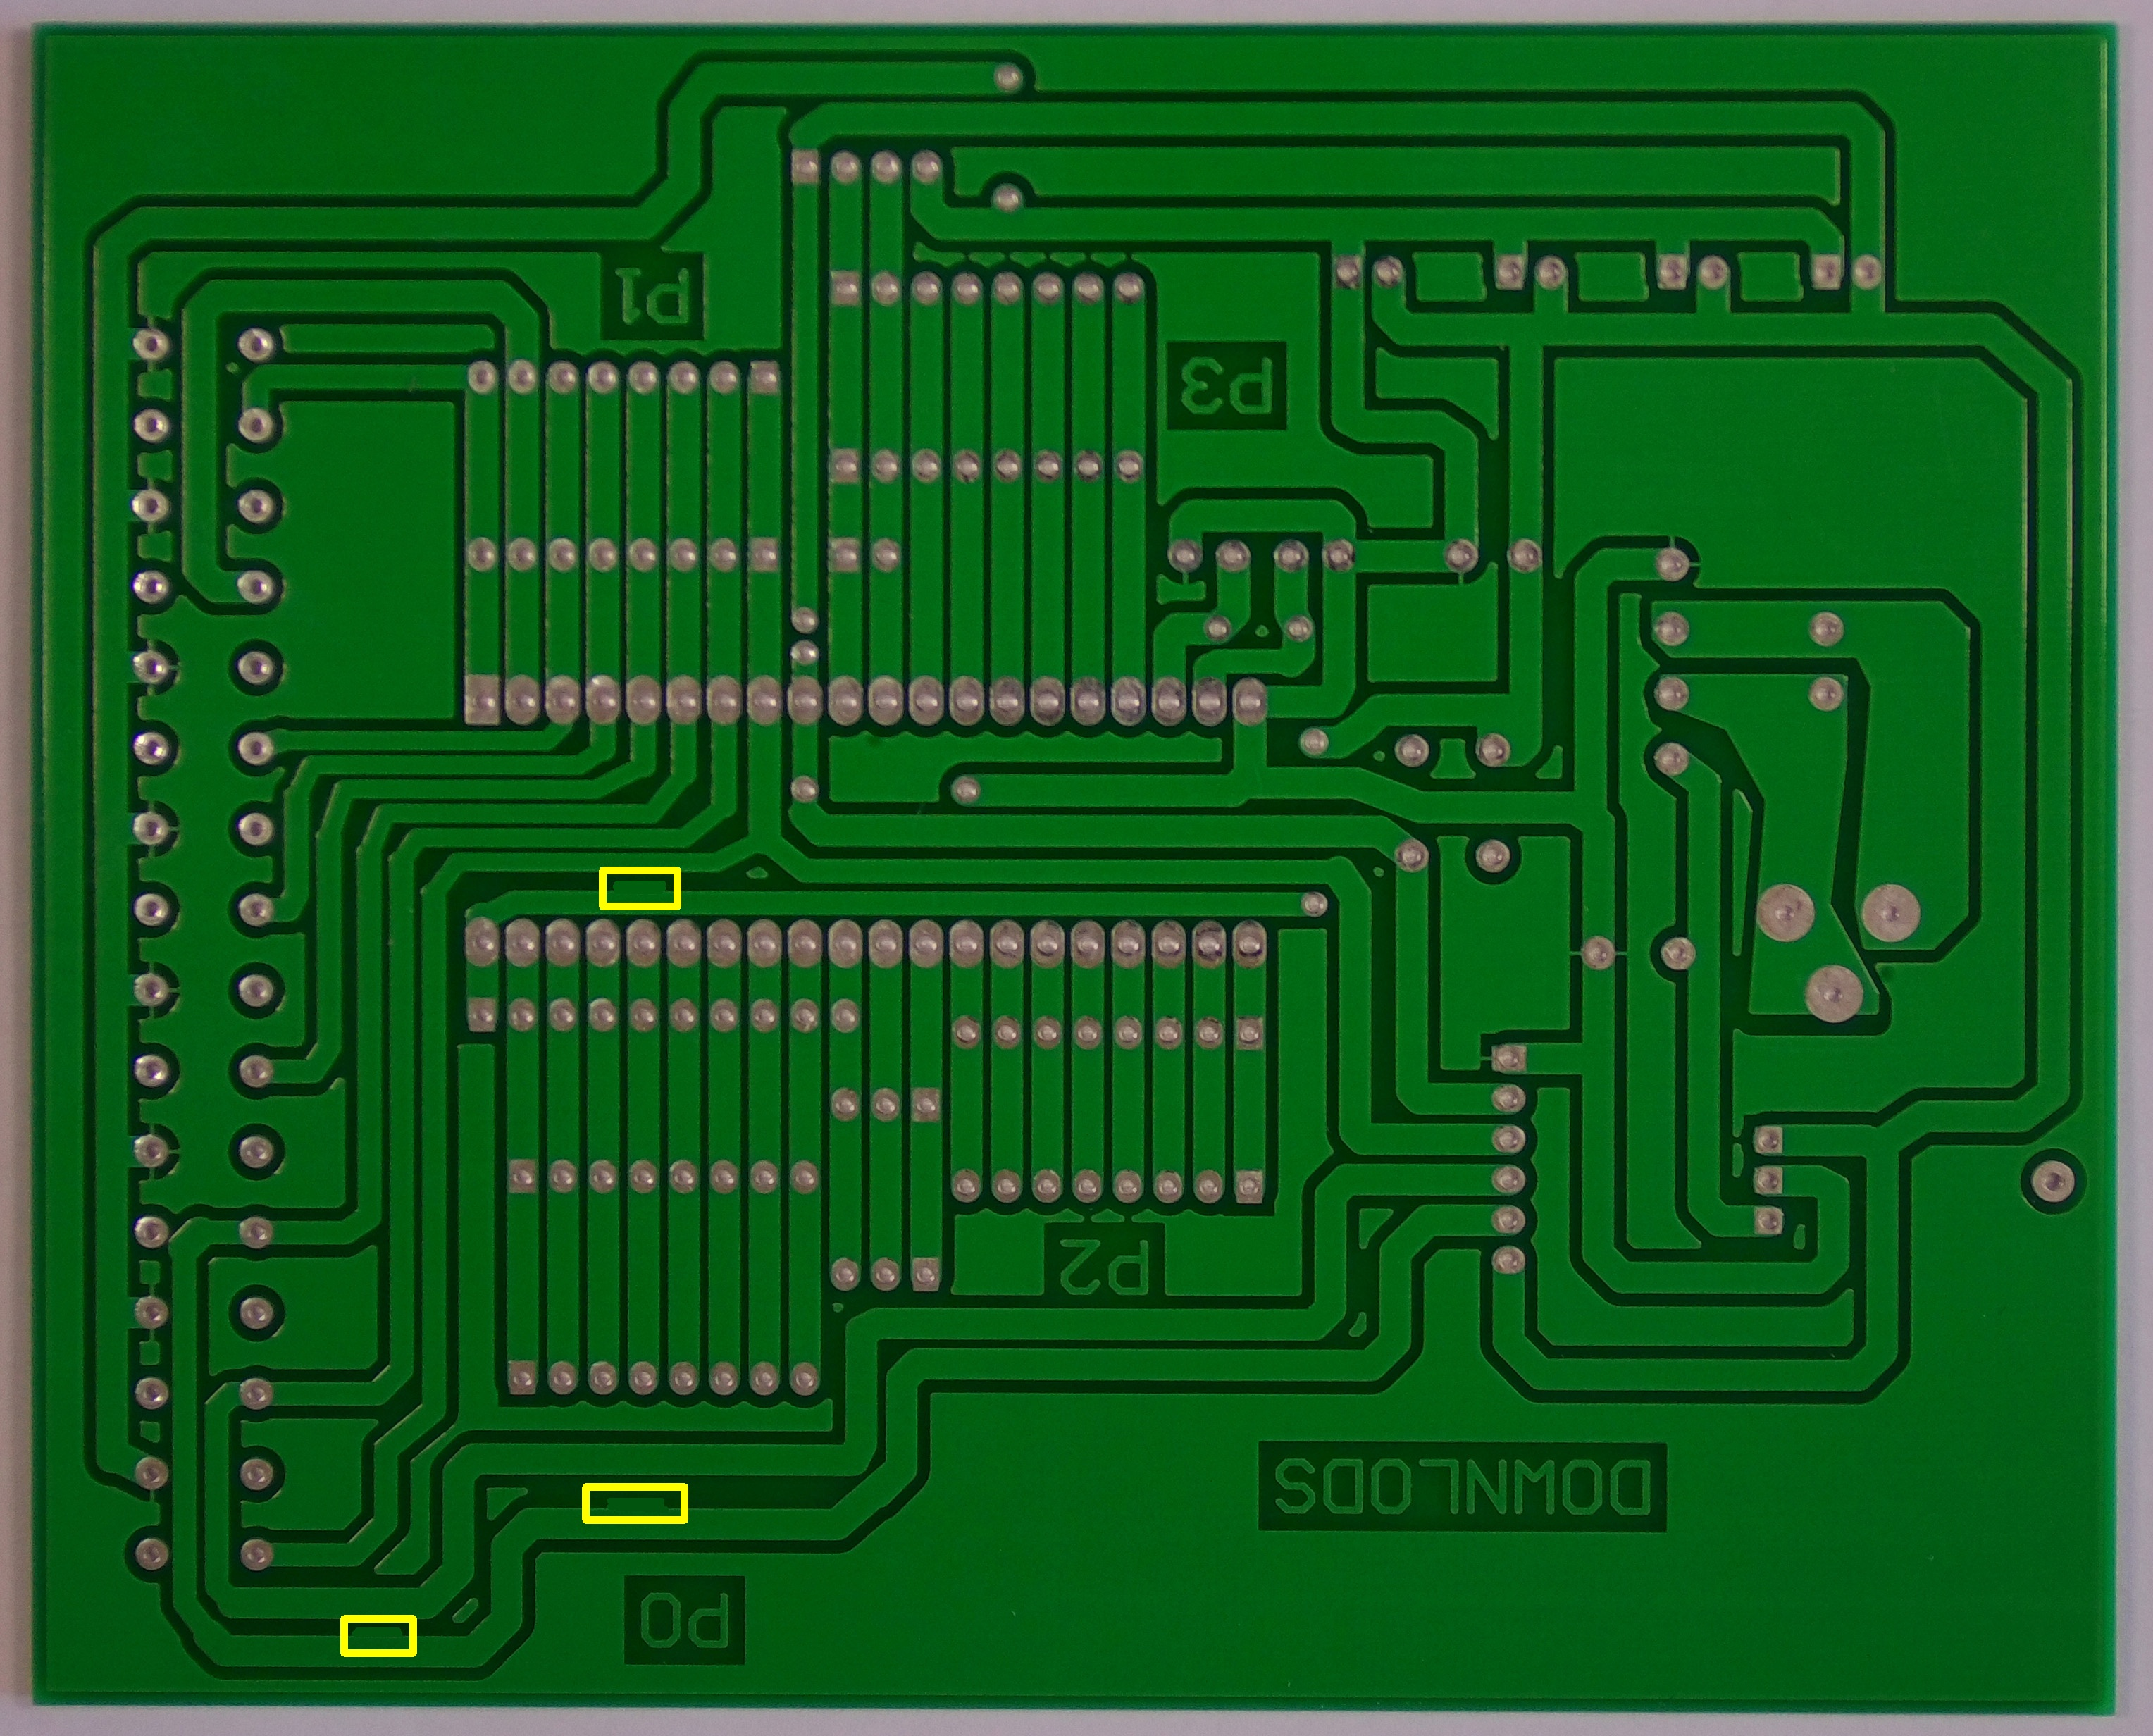}}
    \hfill
    
  \subfloat[MobileViT-XXS: Open Circuit\label{6g}]{%
        \includegraphics[width=0.49\linewidth]{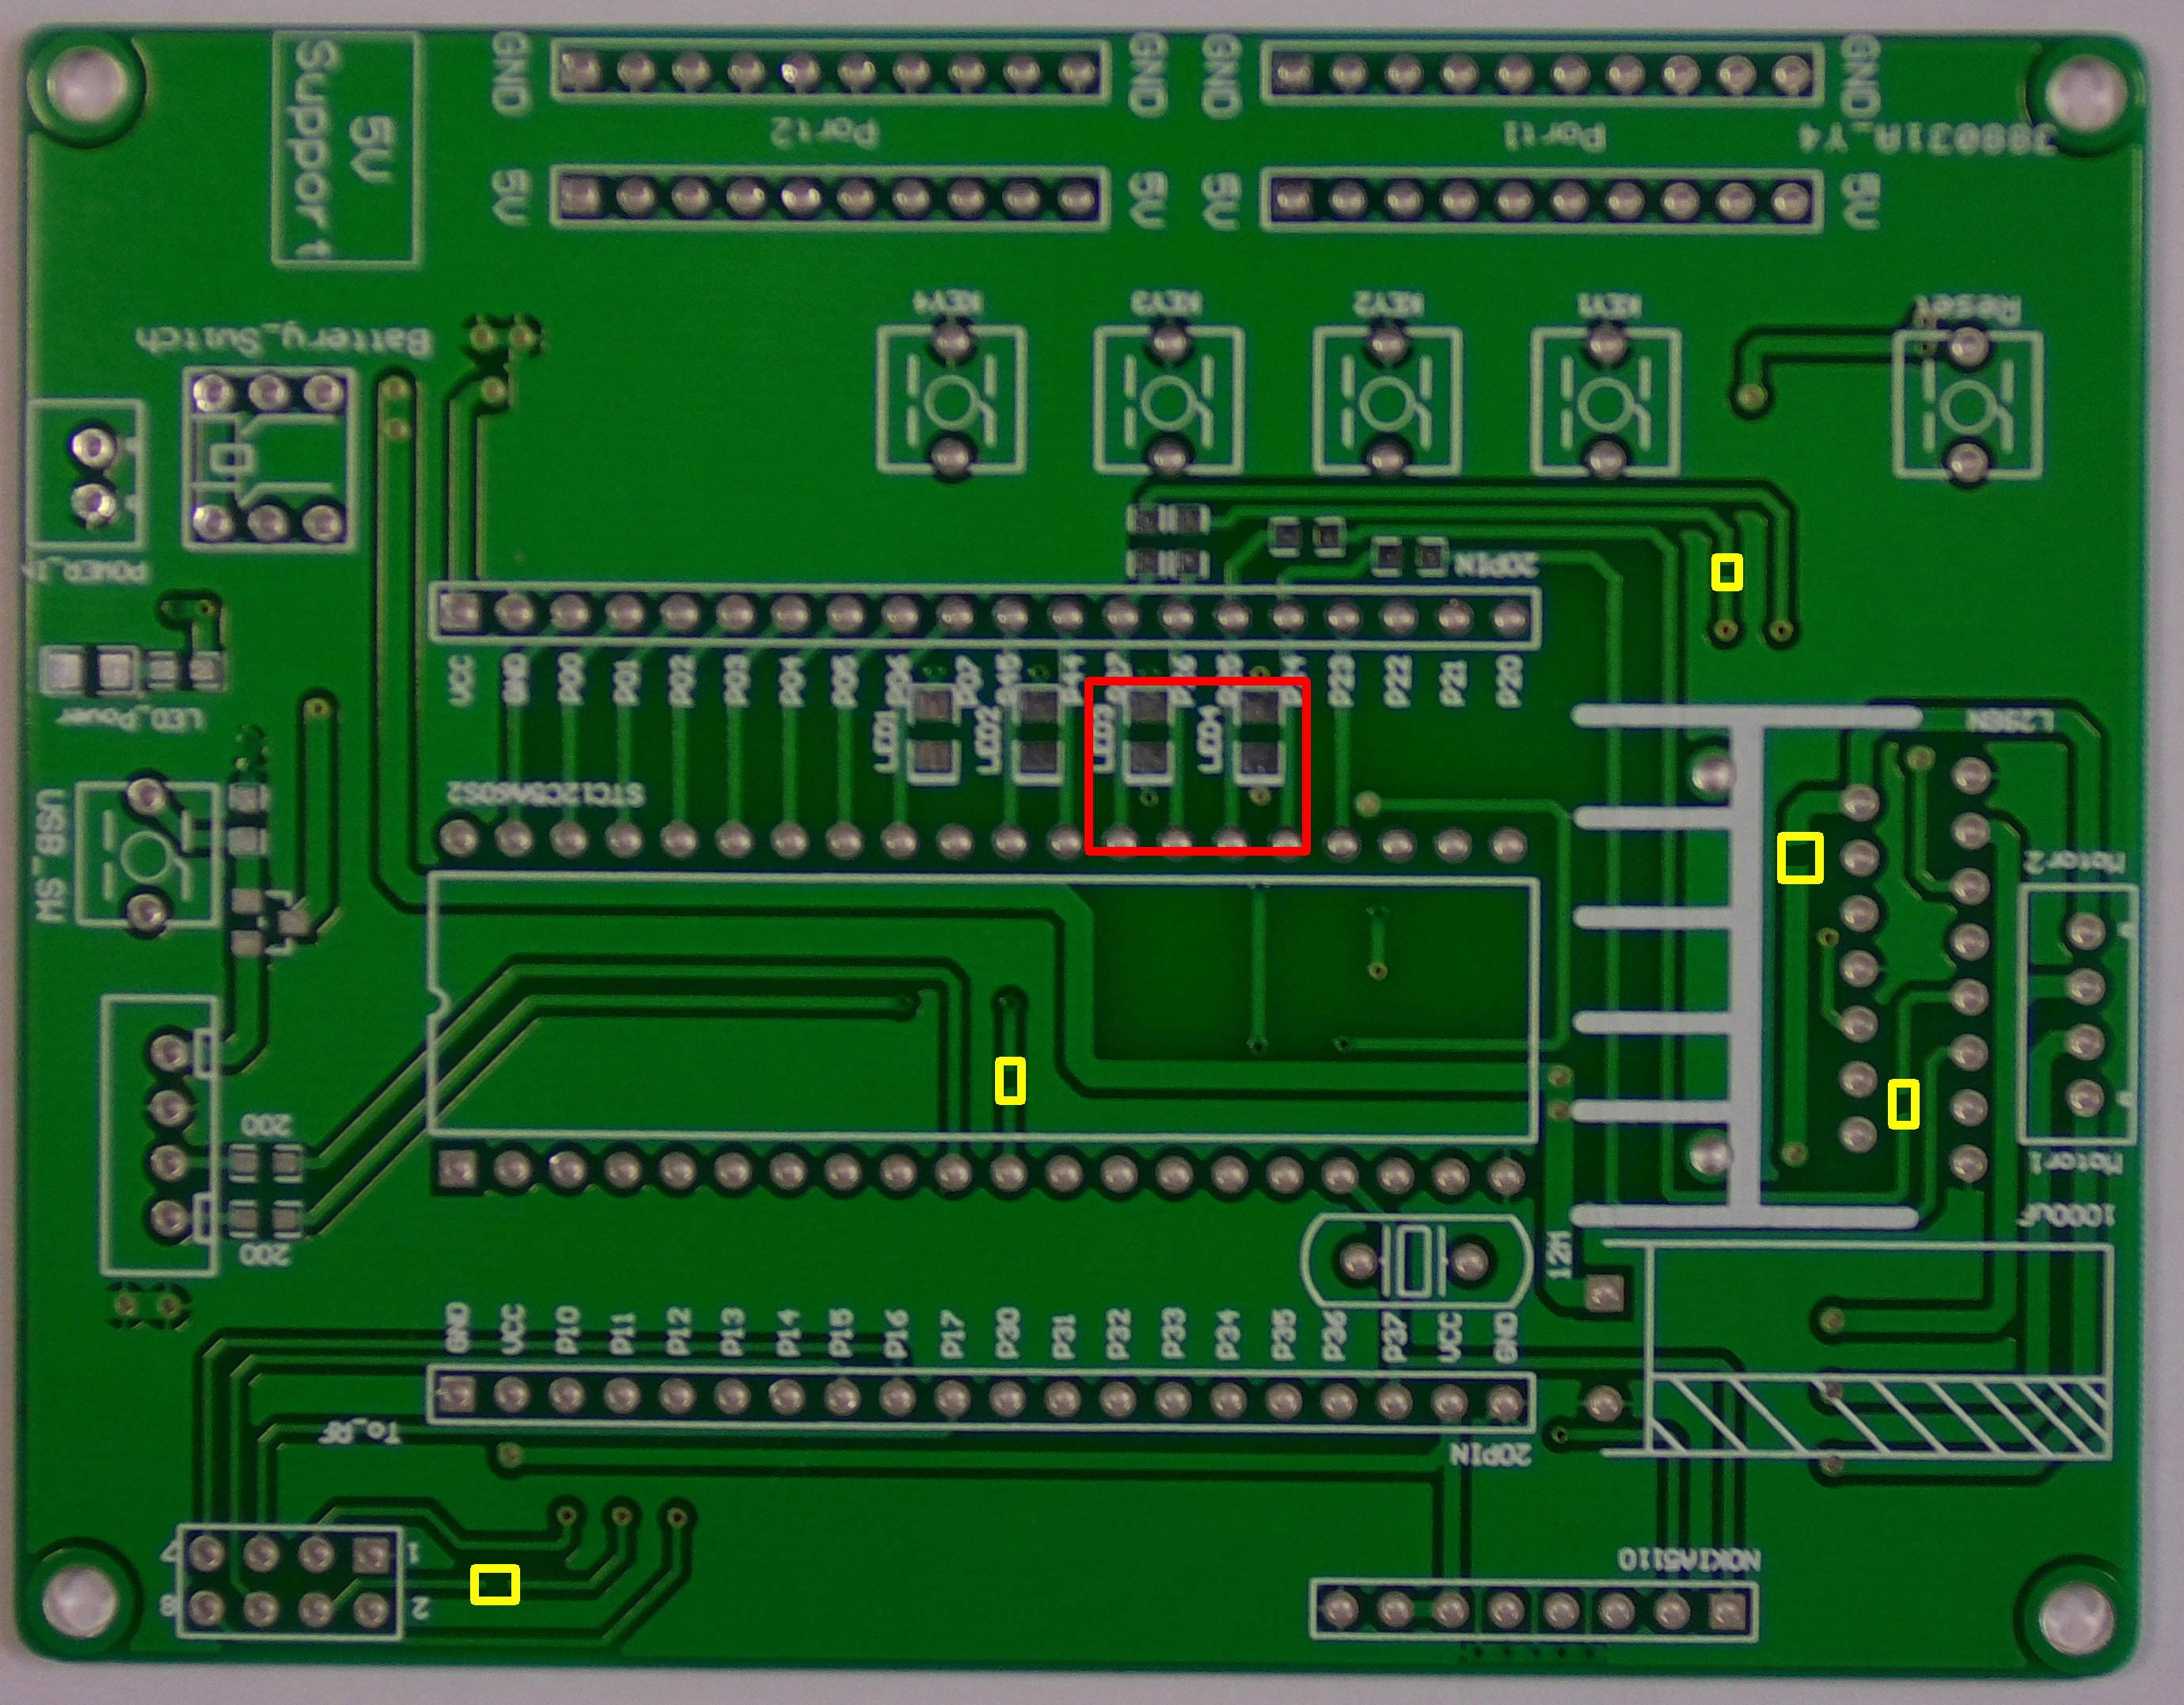}}
    \hfill
    \subfloat[MobileViT-XXS: Spur\label{6h}]{%
        \includegraphics[width=0.48\linewidth]{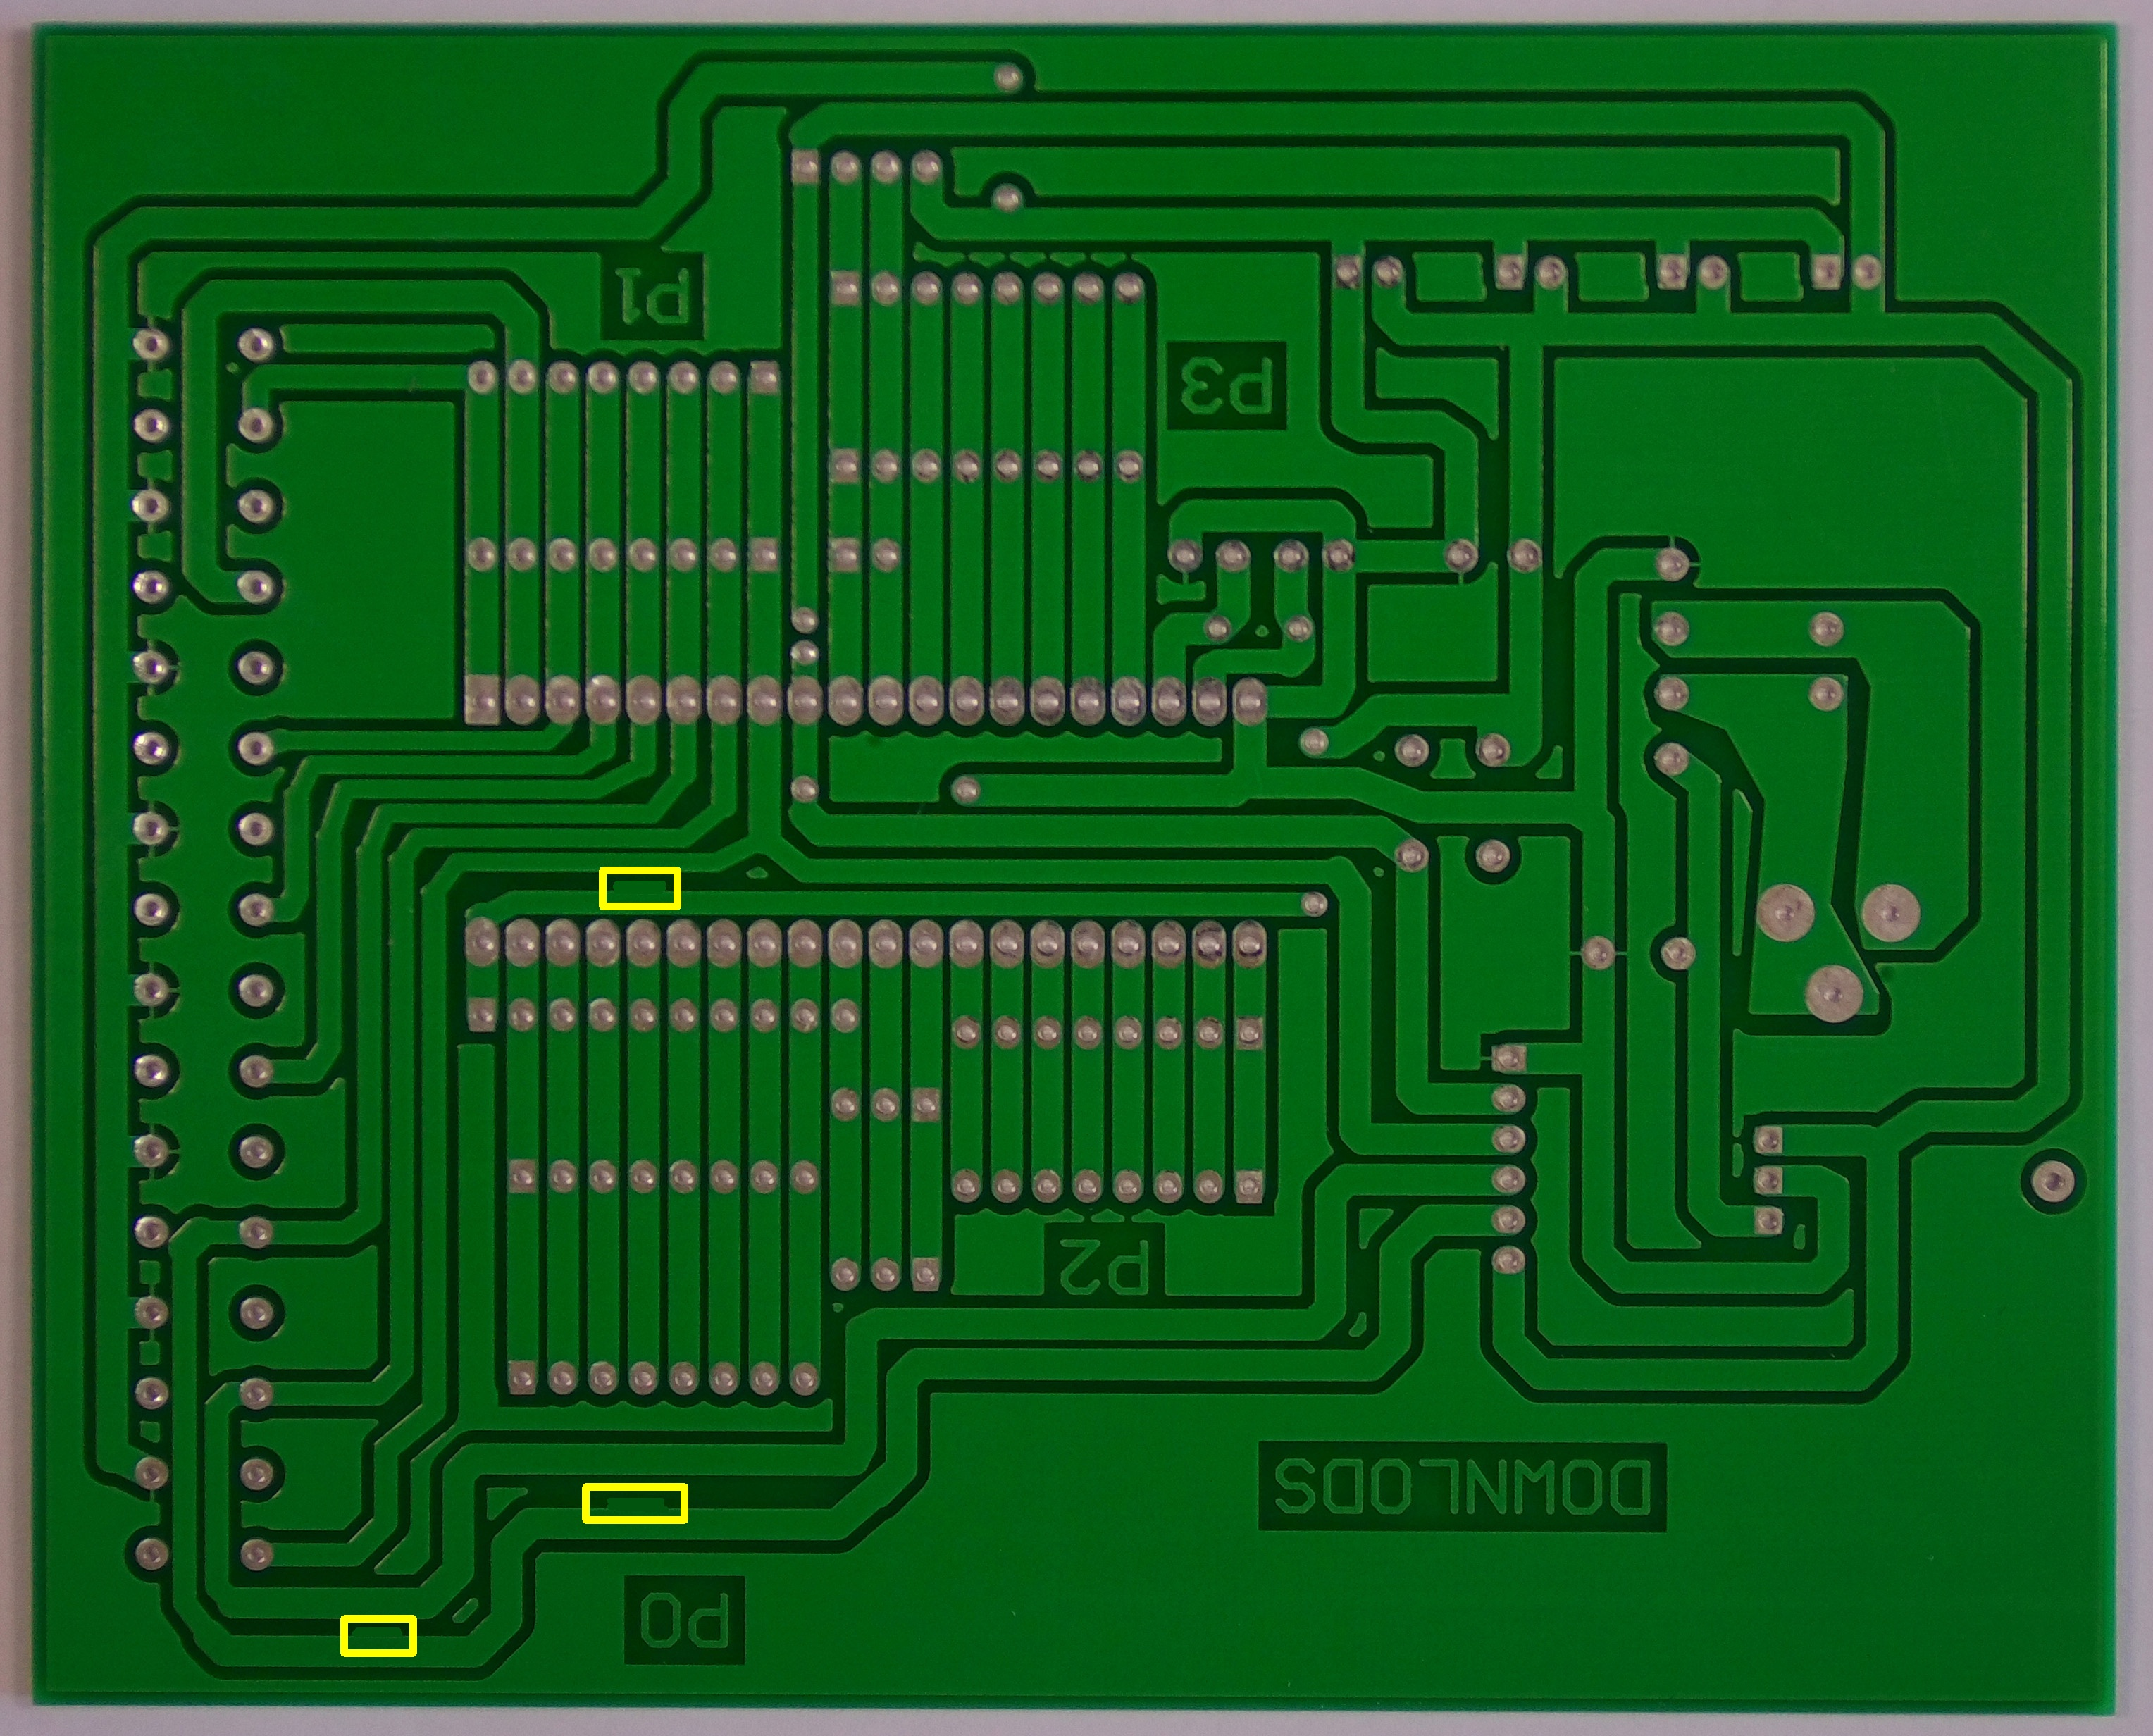}}
    \hfill

  \caption{Result of defect detection on Open Circuit and Spur classes}
  \label{fig:detection_results_OC}
\end{figure}
